# Supplementary material for: High-throughput characterization of transition metal dichalcogenide alloys: Thermodynamic stability and electronic band alignment
Source: arXiv:2204.11223 ancillary file (2022-04-24)
Supplement: Supplementary file 1 [file supporting-information.pdf]

Supporting Information

# High-throughput characterization of transition metal dichalcogenide alloys: Thermodynamic stability and electronic band alignment

Christopher Linderälv, J. Magnus Rahm, and Paul Erhart
Department of Physics, Chalmers University of Technology, SE-41296, Gothenburg, Sweden

## Contents

**Supplementary Notes** **2**
S1. Reference calculations for cluster expansion construction . . . 2
S2. Cluster expansion construction . . . 2
S3. Calculation of critical temperatures and order parameters . . . 2
S4. Electronic structure calculations . . . 3

**Supplementary Tables** **4**
S1. Cluster expansion parameters for M-site mixing alloys . . . 4
S2. Cluster expansion parameters for X-site mixing alloys . . . 5
S3. Boundary phase features . . . 6
S4. Elemental properties . . . 7
S5. Bowing parameters . . . 7

**Supplementary Figures** **8**
S1. Valence band edge position for $HfS_{2x}Se_{2(1-x)}$. . . . 8
S2. Lattice constant as a function of concentration for Mo and W-based alloys (spacegroup 187) . . . 8
S3. Lattice constant as a function of concentration for Hf, Zr and Pd-based alloys (spacegroup 164) . 9
S4. Mixing energies (part 1) for Hf/Mo/Ti/W/Zr-based M-site mixing (spacegroup 187) . . . 10
S5. Mixing energies (part 2) for Hf/Mo/Ti/W/Zr-based M-site mixing (spacegroup 187) . . . 11
S6. Mixing energies for Hf/Mo/Ti/W/Zr-based X-site mixing (spacegroup 187) . . . 12
S7. Mixing energies for Hf/Ti/Zr-based M-site mixing (spacegroup 164) . . . 13
S8. Mixing energies for Hf/Ti/Zr-based X-site mixing (spacegroup 164) . . . 14
S9. Mixing energies for Pd/Pt-based M-site mixing (spacegroup 164) . . . 14
S10. Mixing energies for Pd/Pt-based X-site mixing (spacegroup 164) . . . 15
S11. Results from MC sampling for Mo/W-based M-site mixing (spacegroup 187) . . . 16
S12. Results from MC sampling for Mo/Ti-based M-site mixing (spacegroup 187) . . . 17
S13. Results from MC sampling for Mo-based X-site mixing (spacegroup 187) . . . 18
S14. Results from MC sampling for W-based X-site mixing (spacegroup 187) . . . 19
S15. Results from MC sampling for Hf/Zr-based M-site mixing (spacegroup 164) . . . 20
S16. Results from MC sampling for Hf/Ti-based M-site mixing (spacegroup 164) . . . 21
S17. Results from MC sampling for Ti/Zr-based M-site mixing (spacegroup 164) . . . 22
S18. Results from MC sampling for Hf-based X-site mixing (spacegroup 164) . . . 23
S19. Results from MC sampling for Zr-based X-site mixing (spacegroup 164) . . . 24
S20. Results from MC sampling for Pd/Pt-based M-site mixing (spacegroup 164) . . . 25
S21. Results from MC sampling for Pd-based X-site mixing (spacegroup 164) . . . 26
S22. Results from MC sampling for Pt-based X-site mixing (spacegroup 164) . . . 27

**Supplementary References** **28**

# Supplementary Notes

## Supplementary Note S1: Reference calculations for cluster expansion construction

To generate reference data for the construction of alloy cluster expansions (CEs) (Supplementary Note S2), we carried out density functional theory (DFT) calculations using the projector augmented wave (PAW) method [39] as implemented in the Vienna ab-initio simulation package [40, 41]. The exchange-correlation contribution was represented using the van-der-Waals density functional method [42, 43] with consistent exchange (vdW-DF-cx) [49], which has been shown to be very well suited for transition metal dichalcogenides (TMDs) [44]. The plane-wave cutoff energy was set to 340 eV and we used the PBE PAW setups in version 54. The atomic positions and cell metric were relaxed until residual forces were less than 30 meV Å$^{-1}$ and residual stresses below approximately 2 kbar. Prior to the relaxation, a vacuum region of at least 28 Å was introduced along the direction of the surface normal to minimize interactions between periodic images, and it was asserted that after relaxation the layers were separated by at least 15 Å; in the vast majority of cases it amounted to at least 24 Å. During relaxations the Brillouin zone was sampled with a $\vec{k}$-point density of 0.25 Å$^{-1}$ and first-order Methfessel-Paxton smearing with a width of 0.1 eV. Final energy calculations were carried out for the relaxed structures with a $\vec{k}$-point density of 0.1 Å$^{-1}$ and the tetrahedron method with Blöchl corrections using a smearing width of 0.05 eV.

Structures were generated using the enumeration algorithm introduced in Ref. 45 as implemented in ICET [37]. Calculations were carried out for at least 27 structures (all structures with up to 15 atoms) and at least 28 structures (all structures up to 9 atoms) for M and X-site mixing, respectively. The sufficiency of this data set size was confirmed by testing the convergence for five systems with up to 100 structures, which showed an insignificant improvement in model accuracy.

The DFT data used for CE construction is provided in the form of ASE databases in the ZENODO data set associated with this publication [? ].

## Supplementary Note S2: Cluster expansion construction

In this work, CEs were constructed using the ICET package [37]. In the alloy CE approach, the mixing energy of an interacting many-body system can be expanded in cluster functions as

$$\Delta E_{\mathrm{mix}}(\sigma) = \sum_{\alpha} m_\alpha J_\alpha \langle \Gamma(\sigma) \rangle_\alpha, \tag{1}$$

where $\alpha$ is the index of an orbit (or representative cluster), $m_\alpha$ is the multiplicity of the orbit, $\Gamma$ are cluster functions, $\vec{\sigma}$ denotes the occupation vector, and $J_\alpha$ are the so-called effective cluster interactions (ECIs) that are fitted to DFT data. As a result of the nearsightedness of atomic interactions, the magnitude of the ECIs quickly decay with distance and expansion order, which allows one to truncate the expansion. Here, we considered clusters with one, two, and three sites (singlets, pairs and triplets) in addition to the empty cluster (zerolet). For each alloy system, we then constructed series of CEs with an increasing number of pair and triplet terms. Each individual CE was fitted using the automatic relevance detection regression approach and the default hyperparameters as implemented in SCIKIT-LEARN 1.0 [38]. Among the set of CEs, we selected the one that minimized the Bayesian information criterion (BIC) score, while ensuring a high $R^2$ value for the validation set and a reasonable number of ECIs. In the majority of the systems, triplet clusters were not needed to achieve a satisfactory CE. Cutoffs, cross-validation scores, and other key quantities are summarized in Table S1 and Table S2. Generally the average root mean square errors over the validation sets are (i.e. the cross-validation scores) are very low and the coefficient of determination $R^2$ is very close to 1. The largest errors are obtained for systems with M-site mixing that combine species from the groups 4 (Ti, Zr, Hf) and 6 (Mo, W) of the period table, which also exhibit a very wide range of mixing energies and are very immiscible as indicated by their high critical temperatures. All CEs used in production are also included in the ZENODO data set associated with this publication [? ].

## Supplementary Note S3: Calculation of critical temperatures and order parameters

The alloy CEs were sampled via Monte Carlo (MC) simulations using the MCHAMMER module of the ICET package [37], in order to calculate critical temperatures. To this end, supercells with approximately 1,500 primitive cells were constructed and randomly populated with equal amounts of the two alloyants (50% concentration). These shape of the supercells were chosen in order to accommodate the ground state at 50% concentration. Simulations in the canonical ensemble were commenced at 5000 K and the temperature was lowered in steps of 10 K after 50 MC sweeps (1 MC sweep = $N$ steps, where $N$ is the number of atoms in the supercell), using

the last configuration at one temperature as the starting configuration of the next. Thereafter, MC simulations were continued in parallel for a total of 3,000 MC sweeps at each temperature, and finally 30,000 MC sweeps were carried out at all temperatures within 250 K of the critical temperature. To allow for equilibration, the first 1000 MC sweeps were discarded before data collection.

Critical temperatures $T_C$ were estimated as the temperature with maximum heat capacity $C$, calculated using the variance of the potential energy $E$ according to $C = \left(\langle E^2\rangle - \langle E\rangle^2\right)/k_\mathrm{B}T^2$. We also confirmed that this peak coincided with a rapid decrease of the relevant order parameter, here chosen as the Warren–Cowley short-range order parameter [46] for nearest-neighbor pairs in non-mixing systems, long-range order calculated as structure factors with the relevant $\mathbf{q}$ vector for ordering systems, and the difference in composition between upper and lower layer for Janus systems; all normalized to yield an order parameter of 1 in the perfectly ordered system.

## Supplementary Note S4: Electronic structure calculations

We assessed the variation of band gaps and band edge positions with composition for 48 out of the 72 alloys considered in this work. To this end, we employed special quasi-random structures (SQSs) [47] to mimic complete (fully random) mixing that were generated using the algorithm described in Ref. 48 as implemented in ICET [37], yielding structures contained between 24 and 48 atoms. DFT calculations were again carried out using the PAW method [39] as implemented in the Vienna ab-initio simulation package [40, 41].

For structural relaxations, the exchange-correlation contribution was represented using the vdW-DF-cx method [42, 43, 49] as before (Supplementary Note S1). The plane-wave cutoff energy was set to 340 eV and we used the PBE PAW setups in version 54. The lattice constants were linearly interpolated between the boundary phases, which is motivated by the very small deviations from Vegard's rule that are apparent from the results for enumerated structures (Figure S2, Figure S3). The atomic positions were relaxed at fixed cell metric until residual forces were less than 30 meV Å$^{-1}$. Prior to the relaxation, a vacuum region of at least 28 Å was introduced along the direction of the surface normal to minimize interactions between periodic images, and it was asserted that after relaxation the layers were separated by at least 15 Å; in the vast majority of cases it amounted to at least 24 Å. During relaxations the Brillouin zone was sampled with a $\vec{k}$-point density of 0.25 Å$^{-1}$ and first-order Methfessel-Paxton smearing with a width of 0.1 eV.

We then calculated band gaps and band edge positions for all boundary phases as well as selected SQSs using the HSE06 hybrid exchange-correlation functional [50, 51], which is expected to provide a much improved description of band gaps and band edge positions. Comparison of the results from HSE06 and vdW-DF-cx calculations (Figure S1) shows that the difference can be well approximated by a rigid shift. Given the very high computational cost of the hybrid calculations, we therefore resorted to a simple interpolation procedure for the majority of the alloys. Specifically, the band edge variations were computed as

$$\varepsilon_x = \varepsilon_1^{\mathrm{HSE06}} x + (1-x)\varepsilon_0^{\mathrm{HSE06}} - b^{\mathrm{vdW\text{-}DF\text{-}cx}}(1-x)x, \qquad (2)$$

where boundary phases band edges are indexed with 0 and 1.

# Supplementary Tables

**Table S1: Cluster expansion parameters for M-site mixing alloys.** Cutoffs are given in units of the respective lattice parameter $a_0$ and indicate the longest allowed distance between any two atoms in the cluster. The cross-validation score is the average of ten root-mean square errors obtained by splitting the training set into 90% training structures and 10% validation structures, fitting with the former and calculating the root-mean square error of the latter. The $R^2$ score is the average $R^2$ score obtained for the validation structures in the same tenfold split of the training set.

| Formula | Pair cutoff ($a_0$) | Triplet cutoff ($a_0$) | Cross-validation score (meV/formula unit) | $R^2$ | Nonzero ECIs |
|---|---|---|---|---|---|
| Trigonal (T), P$\bar{3}m1$, ITCA number 164 | | | | | |
| $(Ti, Zr)S_2$ | 1.59 | – | 1.8 | 0.99 | 6 |
| $(Ti, Zr)Se_2$ | 1.62 | – | 1.9 | 0.99 | 5 |
| $(Ti, Zr)Te_2$ | 1.85 | – | 1.5 | 0.98 | 6 |
| $(Hf, Ti)S_2$ | 1.55 | – | 1.4 | 0.99 | 6 |
| $(Hf, Ti)Se_2$ | 1.65 | – | 1.4 | 0.99 | 5 |
| $(Hf, Ti)Te_2$ | 1.57 | – | 1.5 | 0.98 | 5 |
| $(Hf, Zr)S_2$ | 2.75 | – | 0.2 | 0.88 | 5 |
| $(Hf, Zr)Se_2$ | 1.87 | – | 0.5 | 0.40 | 4 |
| $(Hf, Zr)Te_2$ | 4.10 | – | 0.9 | 0.87 | 10 |
| $(Pd, Pt)S_2$ | 1.07 | – | 0.3 | 0.52 | 4 |
| $(Pd, Pt)Se_2$ | 0.79 | – | 0.2 | 0.95 | 2 |
| $(Pd, Pt)Te_2$ | 0.73 | – | 0.3 | 0.98 | 3 |
| Hexagonal (H), P$\bar{6}m2$, ITCA number 187 | | | | | |
| $(Ti, Zr)S_2$ | 1.75 | – | 1.6 | 0.99 | 4 |
| $(Ti, Zr)Se_2$ | 1.68 | – | 1.2 | 0.99 | 4 |
| $(Ti, Zr)Te_2$ | 1.57 | – | 0.9 | 0.99 | 5 |
| $(Hf, Ti)S_2$ | 1.75 | – | 1.1 | 0.99 | 5 |
| $(Hf, Ti)Se_2$ | 1.68 | – | 0.8 | 0.99 | 5 |
| $(Hf, Ti)Te_2$ | 1.57 | – | 0.7 | 0.99 | 5 |
| $(Mo, Ti)S_2$ | 1.28 | 0.92 | 14.4 | 0.95 | 4 |
| $(Mo, Ti)Se_2$ | 1.76 | 0.88 | 15.2 | 0.95 | 8 |
| $(Mo, Ti)Te_2$ | 2.86 | – | 17.8 | 0.88 | 6 |
| $(Ti, W)S_2$ | 0.88 | – | 14.1 | 0.95 | 3 |
| $(Ti, W)Se_2$ | 0.84 | – | 16.6 | 0.93 | 2 |
| $(Ti, W)Te_2$ | 1.18 | – | 18.1 | 0.89 | 5 |
| $(Hf, Zr)S_2$ | 1.64 | – | 0.1 | 0.99 | 5 |
| $(Hf, Zr)Se_2$ | 1.58 | – | 0.1 | 0.90 | 6 |
| $(Hf, Zr)Te_2$ | 1.87 | – | 0.2 | 0.70 | 7 |
| $(Mo, Zr)S_2$ | 3.18 | – | 15.3 | 0.97 | 6 |
| $(Mo, Zr)Se_2$ | 1.76 | – | 15.1 | 0.98 | 6 |
| $(Mo, Zr)Te_2$ | 2.86 | 2.00 | 10.5 | 0.97 | 7 |
| $(W, Zr)S_2$ | 1.83 | – | 17.0 | 0.97 | 6 |
| $(W, Zr)Se_2$ | 1.59 | – | 20.0 | 0.96 | 6 |
| $(W, Zr)Te_2$ | 1.65 | – | 15.3 | 0.95 | 5 |
| $(Hf, Mo)S_2$ | 1.83 | – | 17.2 | 0.97 | 6 |
| $(Hf, Mo)Se_2$ | 1.76 | – | 18.6 | 0.96 | 6 |
| $(Hf, Mo)Te_2$ | 2.86 | – | 15.7 | 0.95 | 5 |
| $(Hf, W)S_2$ | 1.83 | – | 17.8 | 0.97 | 6 |
| $(Hf, W)Se_2$ | 1.59 | – | 19.3 | 0.96 | 6 |
| $(Hf, W)Te_2$ | 1.65 | – | 16.2 | 0.95 | 5 |
| $(Mo, W)S_2$ | 2.38 | – | 0.1 | 1.00 | 4 |
| $(Mo, W)Se_2$ | 2.29 | – | 0.1 | 1.00 | 4 |
| $(Mo, W)Te_2$ | 2.14 | 1.43 | 0.0 | 1.00 | 7 |

**Table S2: Cluster expansion parameters for X-site mixing alloys.** Cutoffs are given in units of the respective lattice parameter $a_0$ and indicate the longest allowed distance between two atoms in the cluster. The cross-validation score is the average of ten root-mean square errors obtained by splitting the training set into 90% training structures and 10% validation structures, fitting with the former and calculating the root-mean square error of the latter. The $R^2$ score is the average $R^2$ score obtained for the validation structures in the same tenfold split of the training set.

| Formula | Pair cutoff ($a_0$) | Triplet cutoff ($a_0$) | Cross-validation score (meV/formula unit) | $R^2$ | Nonzero ECIs |
|---|---|---|---|---|---|
| Trigonal (T), P$\bar{3}m1$, ITCA number 164 | | | | | |
| $Ti(S,Se)_2$ | 1.12 | – | 0.7 | 0.98 | 8 |
| $Ti(S,Te)_2$ | 1.29 | 0.86 | 6.7 | 0.92 | 11 |
| $Ti(Se,Te)_2$ | 1.07 | – | 2.3 | 0.95 | 7 |
| $Zr(S,Se)_2$ | 1.19 | – | 0.5 | 0.96 | 6 |
| $Zr(S,Te)_2$ | 1.23 | – | 5.3 | 0.83 | 8 |
| $Zr(Se,Te)_2$ | 1.31 | 1.08 | 1.0 | 0.98 | 13 |
| $Hf(S,Se)_2$ | 2.29 | – | 0.2 | 0.99 | 9 |
| $Hf(S,Te)_2$ | 2.15 | – | 3.4 | 0.91 | 6 |
| $Hf(Se,Te)_2$ | 2.22 | 1.35 | 1.4 | 0.96 | 10 |
| $Pd(S,Se)_2$ | 1.86 | – | 1.0 | 0.98 | 7 |
| $Pd(S,Te)_2$ | 1.91 | – | 7.2 | 0.96 | 5 |
| $Pd(Se,Te)_2$ | 1.91 | – | 2.7 | 0.95 | 6 |
| $Pt(S,Se)_2$ | 2.13 | – | 1.1 | 0.99 | 7 |
| $Pt(S,Te)_2$ | 2.16 | – | 6.5 | 0.98 | 6 |
| $Pt(Se,Te)_2$ | 1.76 | – | 1.9 | 0.98 | 6 |
| Hexagonal (H), P$\bar{6}m2$, ITCA number 187 | | | | | |
| $Ti(S,Se)_2$ | 2.12 | – | 1.0 | 0.99 | 8 |
| $Ti(S,Te)_2$ | 2.27 | – | 17.8 | 0.84 | 8 |
| $Ti(Se,Te)_2$ | 1.16 | – | 2.3 | 0.98 | 9 |
| $Zr(S,Se)_2$ | 2.05 | – | 1.8 | 0.94 | 7 |
| $Zr(S,Te)_2$ | 1.14 | – | 8.7 | 0.94 | 6 |
| $Zr(Se,Te)_2$ | 1.18 | – | 2.0 | 0.98 | 8 |
| $Hf(S,Se)_2$ | 1.24 | – | 0.9 | 0.98 | 6 |
| $Hf(S,Te)_2$ | 2.15 | – | 10.1 | 0.90 | 7 |
| $Hf(Se,Te)_2$ | 2.07 | – | 1.2 | 0.99 | 8 |
| $Mo(S,Se)_2$ | 2.38 | 1.59 | 0.3 | 1.00 | 11 |
| $Mo(S,Te)_2$ | 2.29 | 1.53 | 3.1 | 0.99 | 11 |
| $Mo(Se,Te)_2$ | 2.29 | 1.53 | 0.5 | 1.00 | 11 |
| $W(S,Se)_2$ | 1.37 | 0.92 | 0.3 | 1.00 | 11 |
| $W(S,Te)_2$ | 1.32 | 0.88 | 3.4 | 0.99 | 11 |
| $W(Se,Te)_2$ | 1.32 | 0.88 | 1.3 | 1.00 | 11 |

**Table S3: Boundary phase features.** Data used in the construction of models for the critical temperatures and categorization of X-site alloys. The band edges (VBM and CBM) are computed on the level of conventional DFT. The bulk modulus is computed as the 3D counterpart i.e. $B = (c_{11} + 2c_{12})/3$ and then multiplied by the out-of-plane lattice vector.

| | $a_0$ (Å) | VBM (eV) | CBM (eV) | $B$ (eVÅ$^{-2}$) | Tr($\mathcal{Z}^*_{\mathrm{M}}$) (e) | Tr($\mathcal{Z}^*_{\mathrm{X}}$) (e) |
|---|---|---|---|---|---|---|
| Trigonal (T), P$\bar{3}m1$, ITCA number 164 | | | | | | |
| $HfS_2$ | 3.60 | −6.4 | −5.2 | 250 | 14.1 | −7.0 |
| $HfSe_2$ | 3.72 | −5.5 | −5.1 | 216 | 15.2 | −7.6 |
| $HfTe_2$ | 3.91 | −4.8 | −4.7 | 152 | 16.9 | −8.4 |
| $MoS_2$ | 3.12 | −5.1 | −5.1 | 194 | −12.2 | 6.3 |
| $MoSe_2$ | 3.23 | −4.7 | −4.6 | 240 | −10.3 | 5.2 |
| $MoTe_2$ | 3.45 | −4.4 | −4.3 | 208 | −9.6 | 4.8 |
| $PdS_2$ | 3.50 | −6.4 | −5.1 | 248 | 5.7 | −2.9 |
| $PdSe_2$ | 3.67 | −5.5 | −4.8 | 200 | 4.9 | −2.5 |
| $PdTe_2$ | 3.94 | −4.6 | −4.5 | 165 | 3.3 | −1.6 |
| $PtS_2$ | 3.53 | −6.4 | −4.6 | 289 | 5.0 | −2.5 |
| $PtSe_2$ | 3.70 | −5.8 | −4.4 | 253 | 4.2 | −2.1 |
| $PtTe_2$ | 3.96 | −4.8 | −4.1 | 239 | 2.3 | −1.1 |
| $TiS_2$ | 3.36 | −5.8 | −5.8 | 243 | 14.6 | −7.3 |
| $TiSe_2$ | 3.49 | −5.4 | −5.3 | 197 | 18.8 | −9.4 |
| $TiTe_2$ | 3.68 | −4.9 | −4.8 | 168 | 9.2 | −4.6 |
| $WS_2$ | 3.14 | −5.0 | −4.9 | 168 | −16.3 | 8.2 |
| $WSe_2$ | 3.24 | −4.5 | −4.4 | 248 | −10.8 | 5.4 |
| $WTe_2$ | 3.46 | −4.1 | −4.0 | 193 | −10.6 | 5.3 |
| $ZrS_2$ | 3.64 | −6.5 | −5.4 | 233 | 14.5 | −7.3 |
| $ZrSe_2$ | 3.75 | −5.6 | −5.2 | 202 | 16.0 | −8.0 |
| $ZrTe_2$ | 3.90 | −5.0 | −4.9 | 126 | 15.3 | −7.7 |
| Hexagonal (H), P$\bar{6}m2$, ITCA number 187 | | | | | | |
| $HfS_2$ | 3.50 | −7.0 | −5.9 | 348 | 9.6 | −4.8 |
| $HfSe_2$ | 3.62 | −6.4 | −5.6 | 295 | 10.0 | −5.0 |
| $HfTe_2$ | 3.85 | −5.5 | −5.3 | 216 | 12.8 | −6.4 |
| $MoS_2$ | 3.15 | −6.0 | −4.2 | 432 | −2.4 | 1.2 |
| $MoSe_2$ | 3.28 | −5.4 | −3.9 | 358 | −3.9 | 2.0 |
| $MoTe_2$ | 3.50 | −5.0 | −3.8 | 284 | −6.9 | 3.4 |
| $TiS_2$ | 3.30 | −6.9 | −6.1 | 321 | 9.5 | −4.8 |
| $TiSe_2$ | 3.45 | −6.2 | −5.7 | 279 | 10.2 | −5.1 |
| $TiTe_2$ | 3.68 | −5.3 | −5.3 | 196 | 19.5 | −9.7 |
| $WS_2$ | 3.15 | −5.8 | −3.9 | 471 | −1.2 | 0.6 |
| $WSe_2$ | 3.28 | −5.2 | −3.5 | 368 | −2.7 | 1.3 |
| $WTe_2$ | 3.50 | −4.8 | −3.6 | 278 | −5.5 | 2.8 |
| $ZrS_2$ | 3.53 | −6.9 | −6.0 | 321 | 9.7 | −4.9 |
| $ZrSe_2$ | 3.66 | −6.4 | −5.6 | 275 | 10.0 | −5.0 |
| $ZrTe_2$ | 3.86 | −5.6 | −5.3 | 205 | 13.6 | −6.8 |

**Table S4: Elemental properties.** Elemental properties of considered elements. The electronegativity ($\chi$) scale is the Pauling scale and the covalent radius ($r_c$) is in units of pm.

| | $\chi$ | $r_c$ (pm) |
|---|---|---|
| Mo | 2.16 | 154 |
| W | 2.36 | 162 |
| Zr | 1.33 | 175 |
| Hf | 1.30 | 187 |
| Ti | 1.54 | 160 |
| Pd | 2.20 | 139 |
| Pt | 2.28 | 136 |
| Te | 2.10 | 138 |
| Se | 2.55 | 120 |
| S | 2.58 | 105 |

**Table S5: Bowing parameters.** Bowing parameters for the $MX_{2x}X'_{2(1-x)}$ with M=Mo, W and X, X'=S, Se, Te alloys. Values in parenthesis are from Ref. 20.

| | $b_{\mathrm{VBM}}$ (eV) | $b_{\mathrm{CBM}}$ (eV) |
|---|---|---|
| $MoS_{2x}Se_{2(1-x)}$ | −0.07 (−0.22) | −0.23 (−0.18) |
| $MoSe_{2x}Te_{2(1-x)}$ | −0.22 (−0.36) | −0.11 (−0.24) |
| $MoS_{2x}Te_{2(1-x)}$ | −0.98 (−1.17) | −0.55 (−0.76) |
| $WS_{2x}Se_{2(1-x)}$ | 0.00 (−0.21) | −0.16 (−0.16) |
| $WSe_{2x}Te_{2(1-x)}$ | −0.13 (−0.32) | −0.07 (−0.20) |
| $WS_{2x}Te_{2(1-x)}$ | −0.84 (−1.06) | −0.46 (−0.70) |

# Supplementary Figures

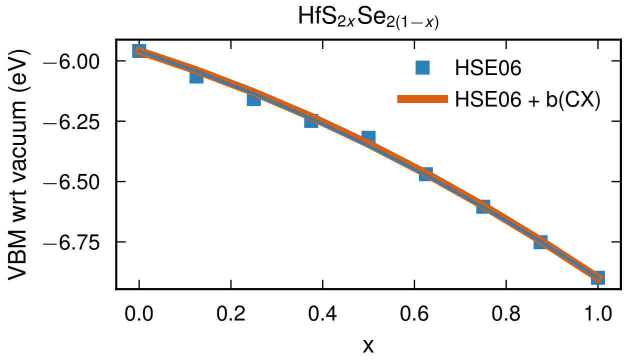


**Figure S1: Valence band edge position for $HfS_{2x}Se_{2(1-x)}$.** Comparison between HSE06 and the band edges from HSE06 with the bowing parameter from vdW-df-cx.

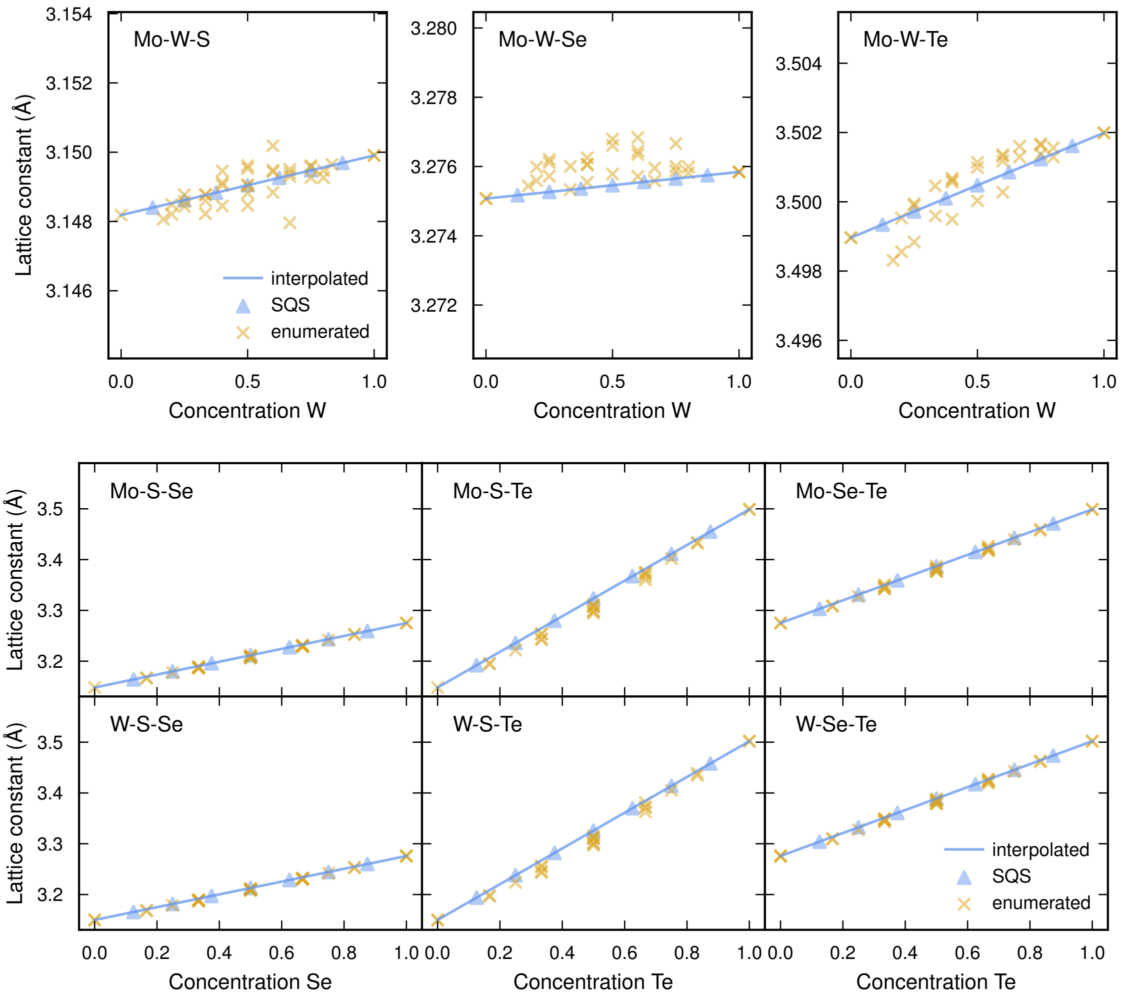


**Figure S2: Lattice constant as a function of concentration for Mo and W-based alloys (spacegroup 187).** top: M-site mixing; bottom: X-site mixing

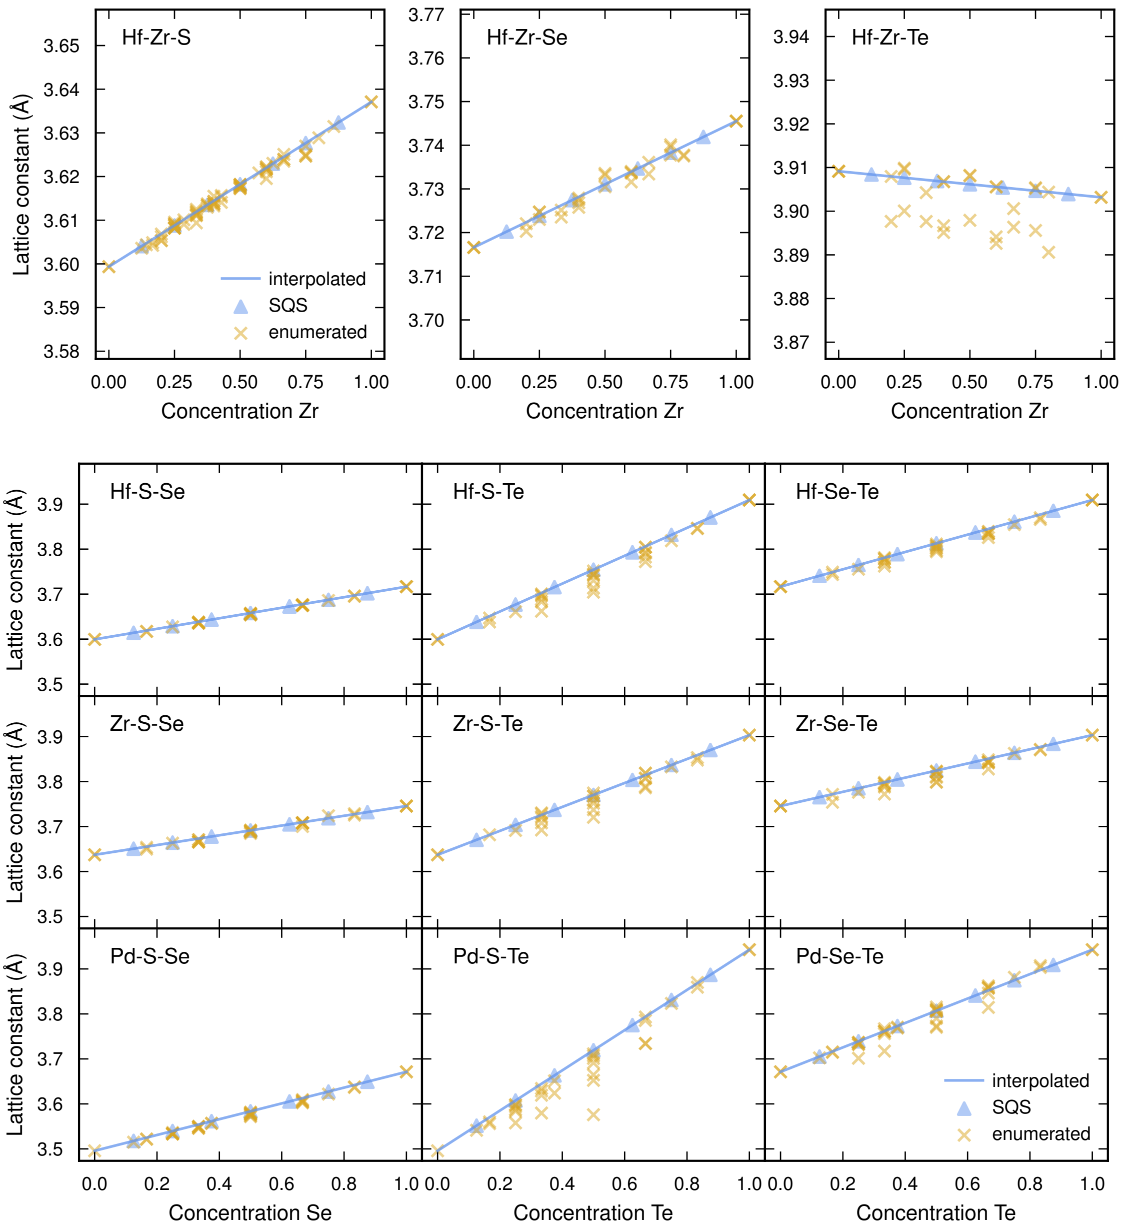


**Figure S3: Lattice constant as a function of concentration for Hf, Zr and Pd-based alloys (space-group 164).** top: M-site mixing; bottom: X-site mixing

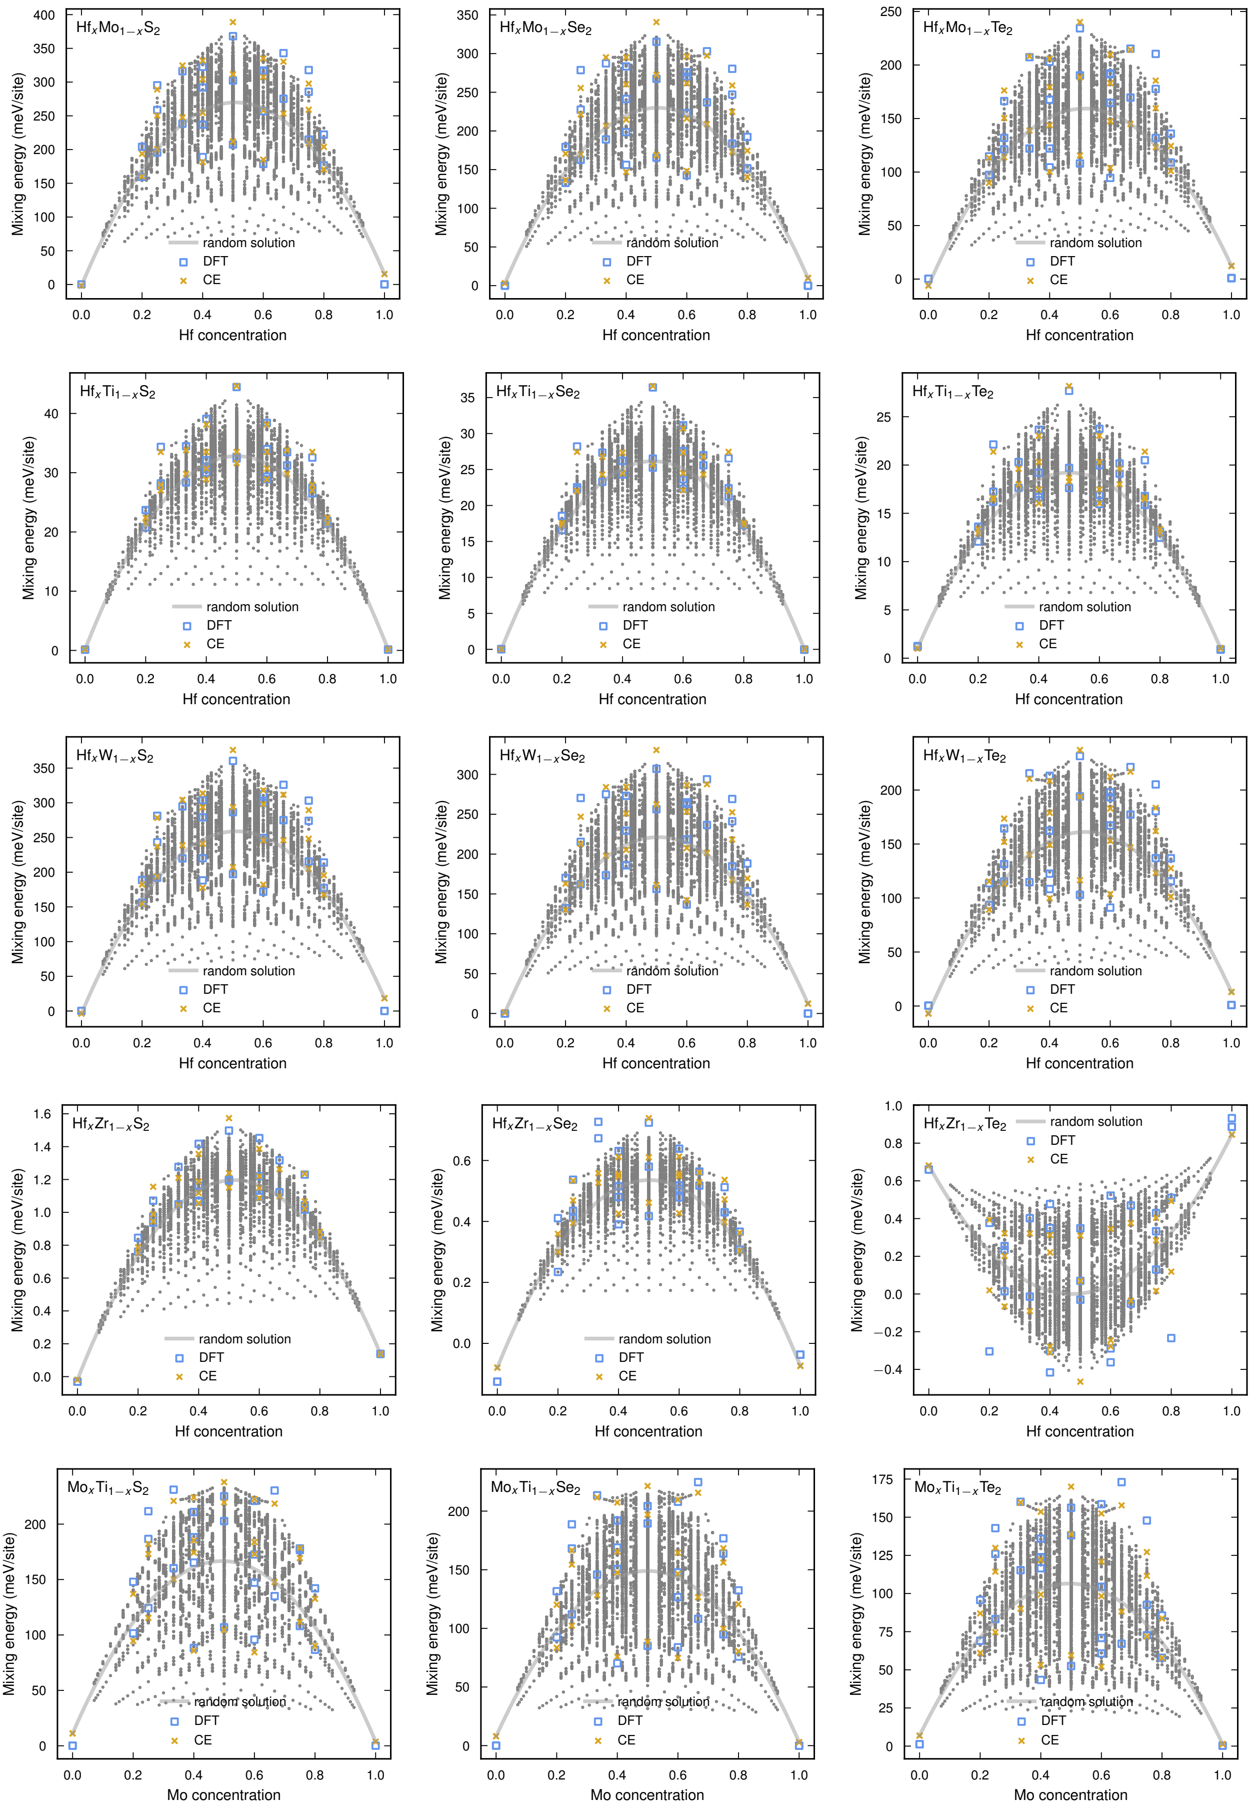


**Figure S4: Mixing energies (part 1) for Hf/Mo/Ti/W/Zr-based M-site mixing (spacegroup 187).** Small gray circles mark mixing energies of enumerated structures obtained using the CE.

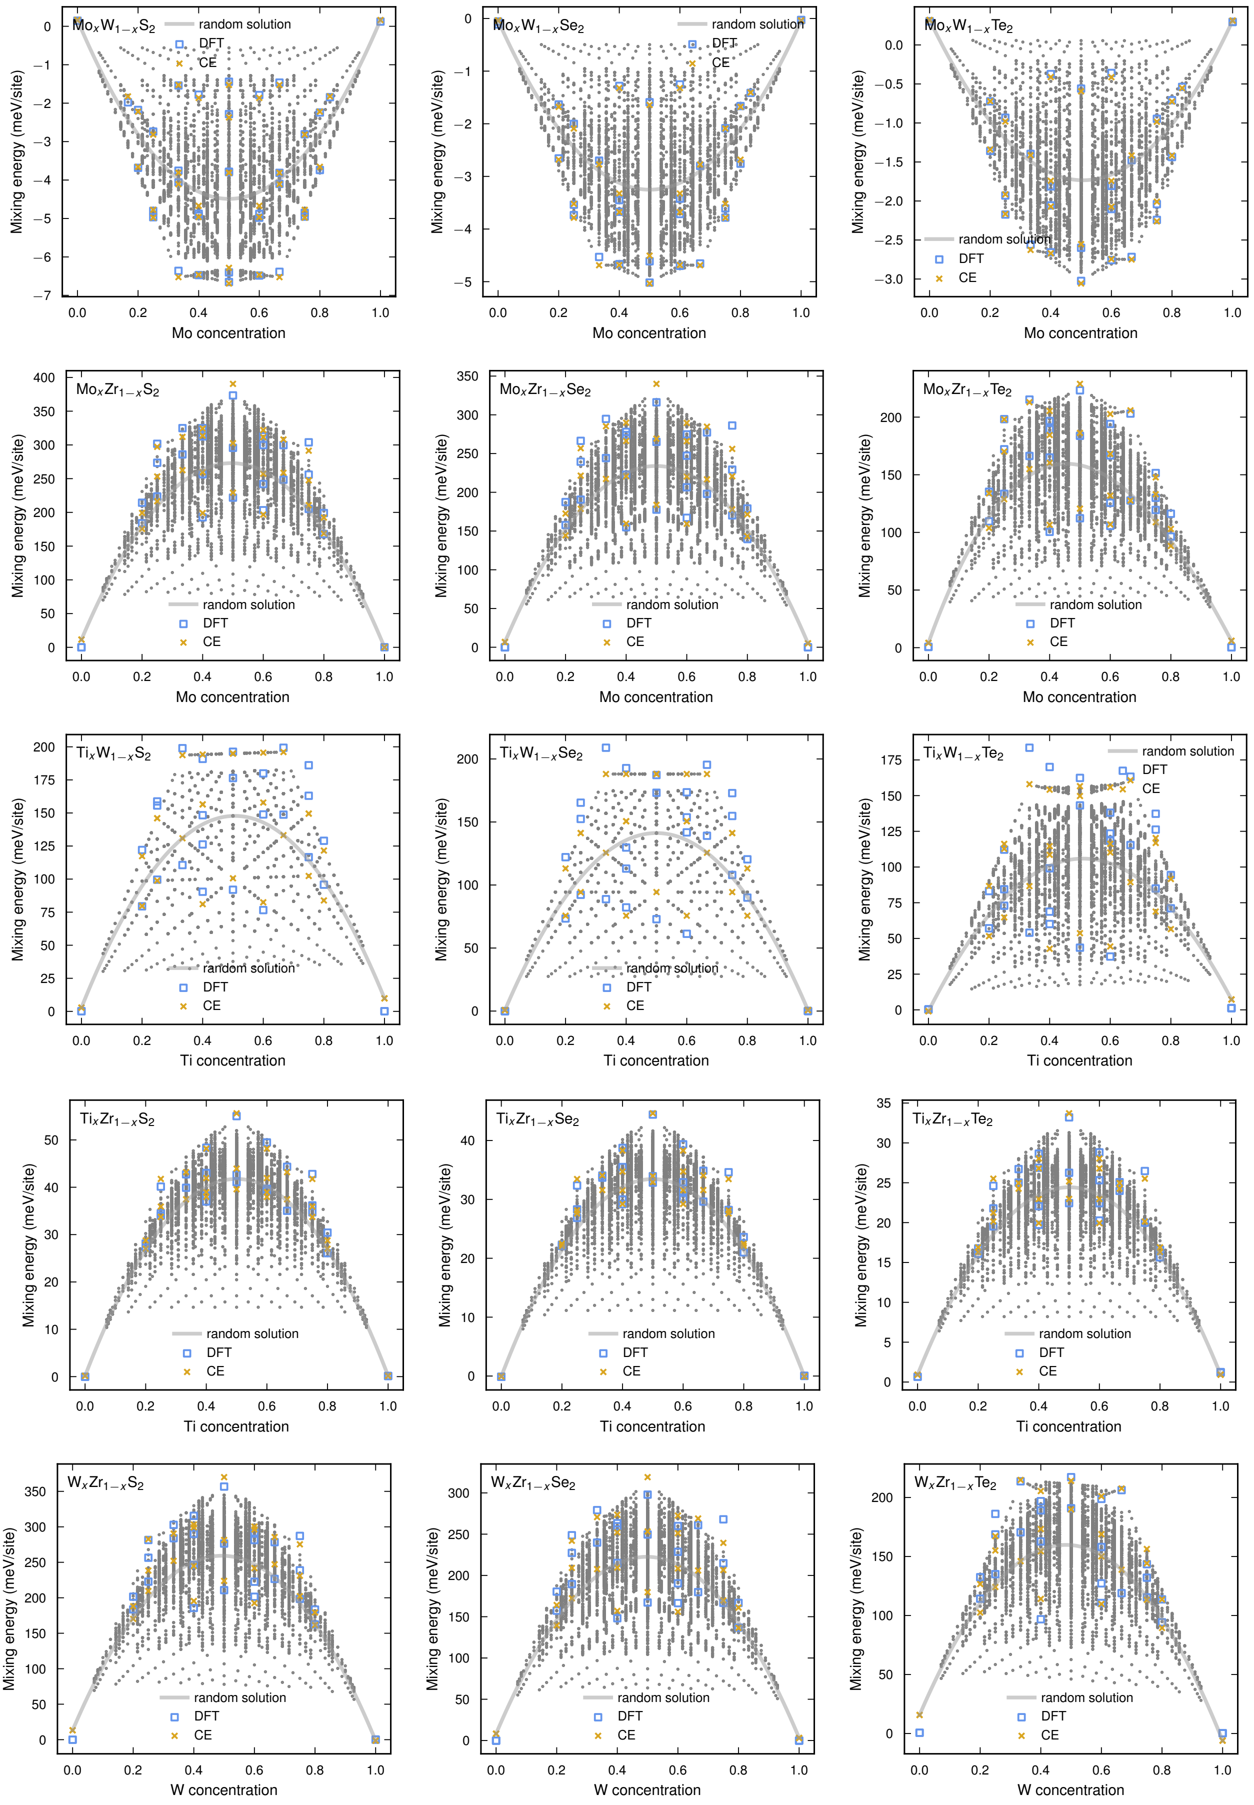


**Figure S5: Mixing energies (part 2) for Hf/Mo/Ti/W/Zr-based M-site mixing (spacegroup 187).** Small gray circles mark mixing energies of enumerated structures obtained using the CE.

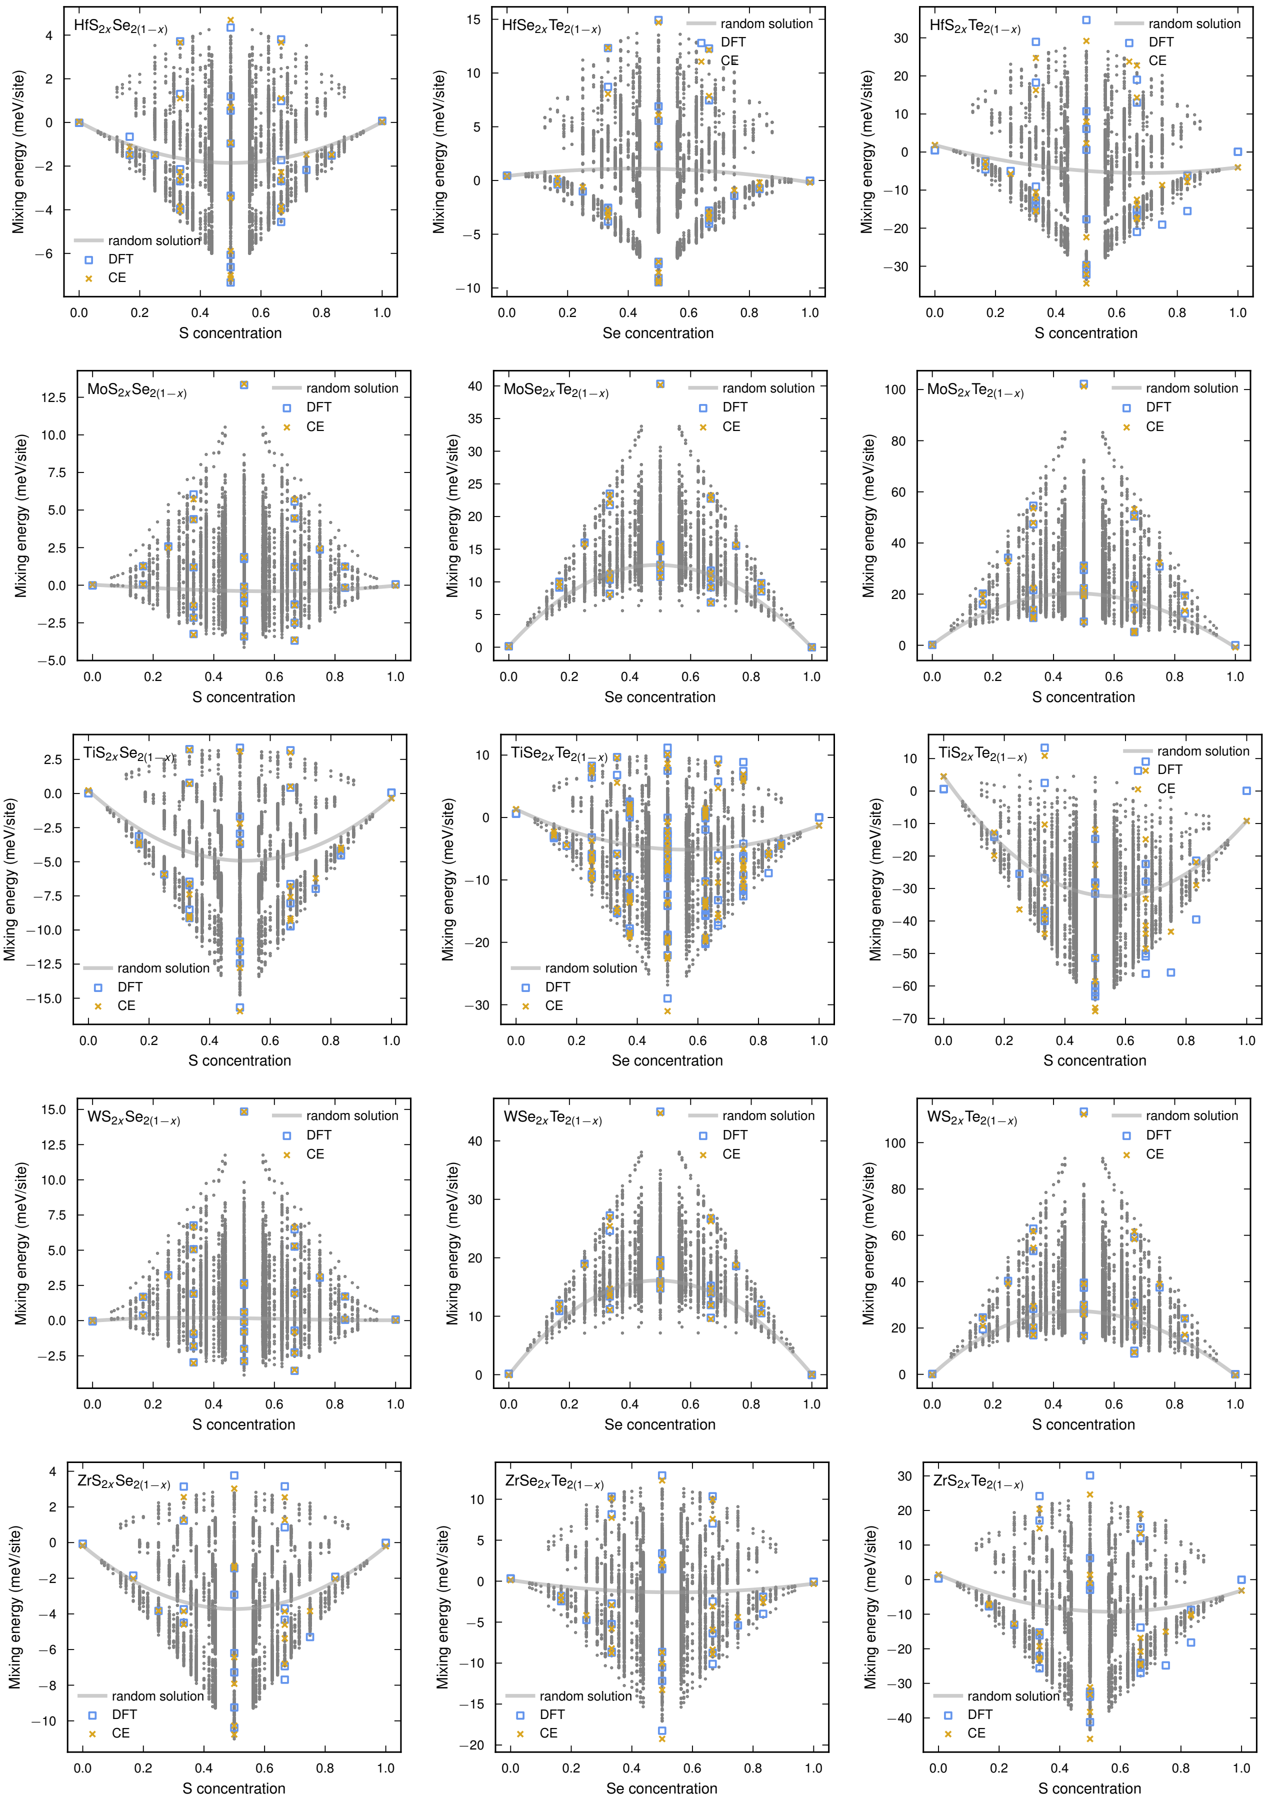


**Figure S6: Mixing energies for Hf/Mo/Ti/W/Zr-based X-site mixing (spacegroup 187).** Small gray circles mark mixing energies of enumerated structures obtained using the CE.

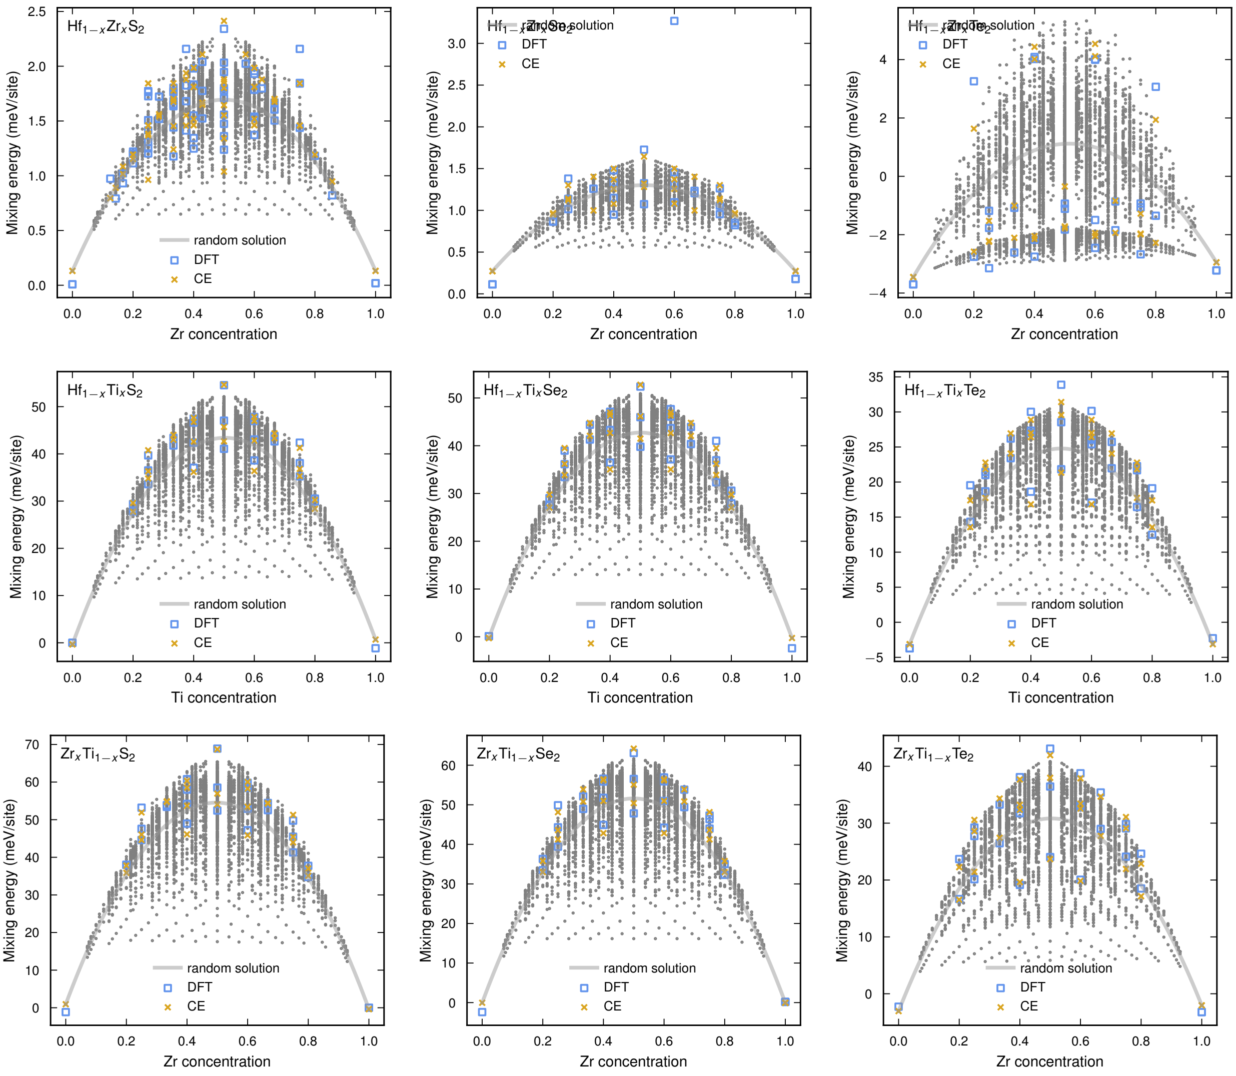


**Figure S7: Mixing energies for Hf/Ti/Zr-based M-site mixing (spacegroup 164).** Small gray circles mark mixing energies of enumerated structures obtained using the CE.

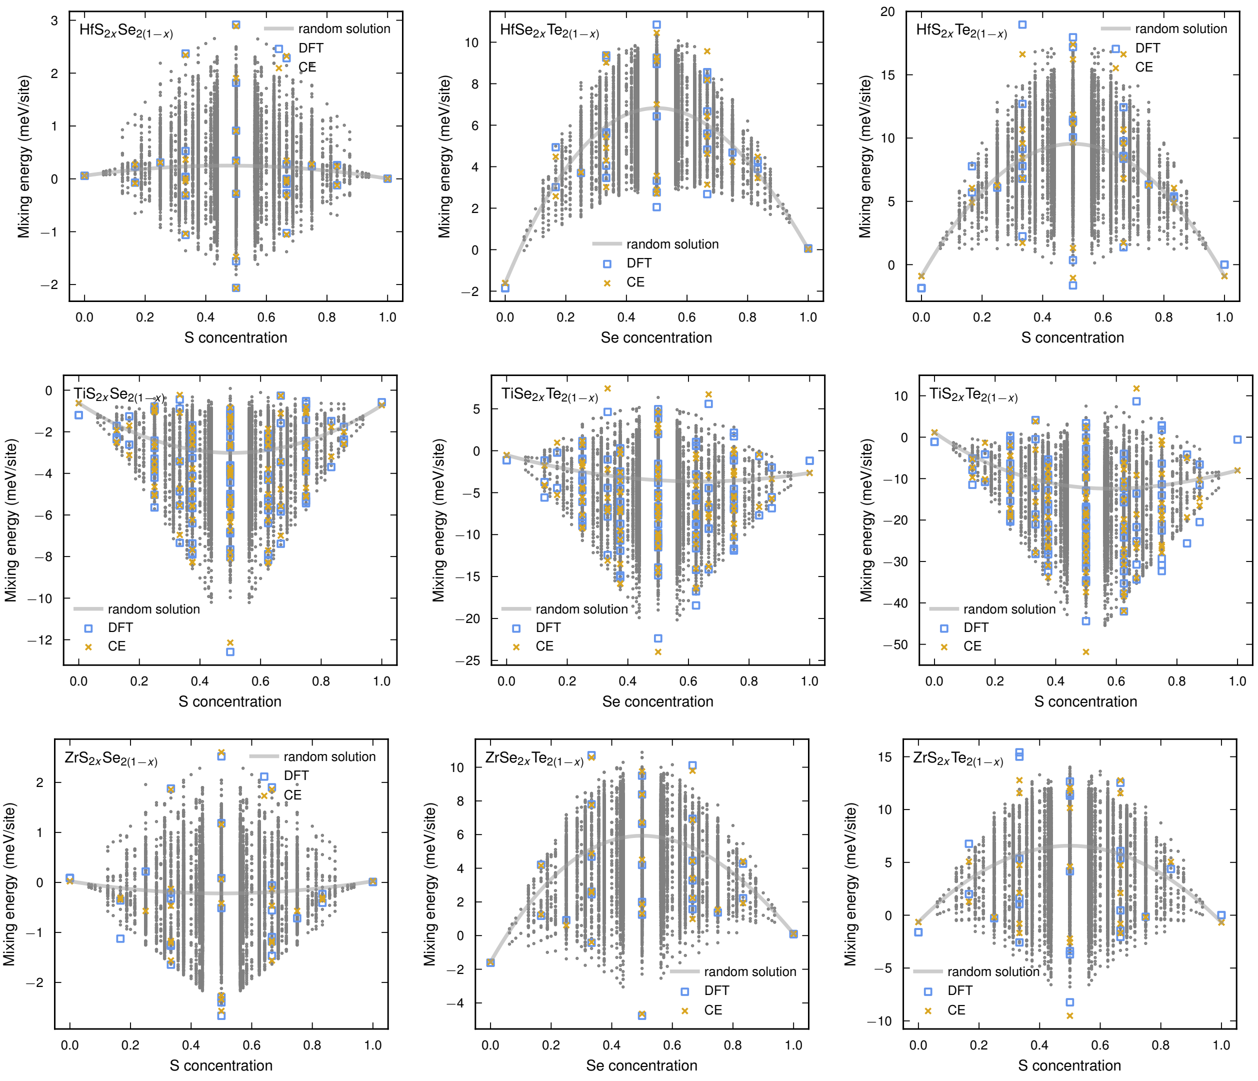


**Figure S8: Mixing energies for Hf/Ti/Zr-based X-site mixing (spacegroup 164).** Small gray circles mark mixing energies of enumerated structures obtained using the CE.

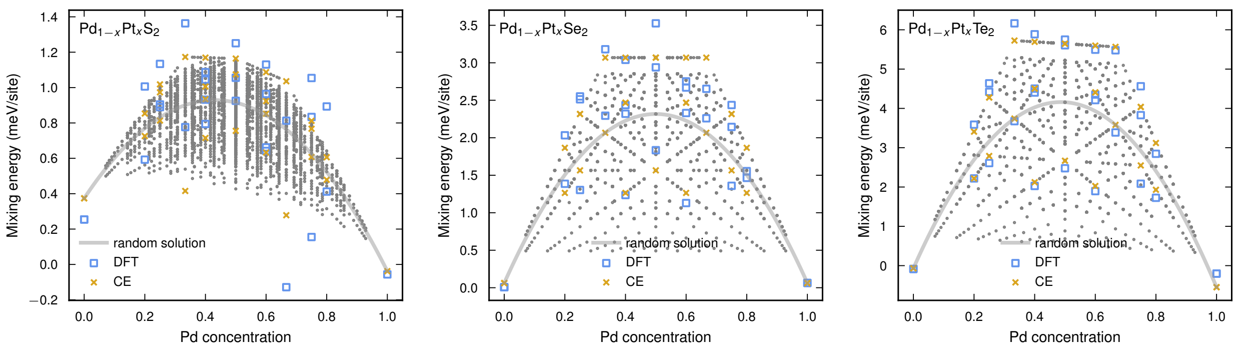


**Figure S9: Mixing energies for Pd/Pt-based M-site mixing (spacegroup 164).** Small gray circles mark mixing energies of enumerated structures obtained using the CE.

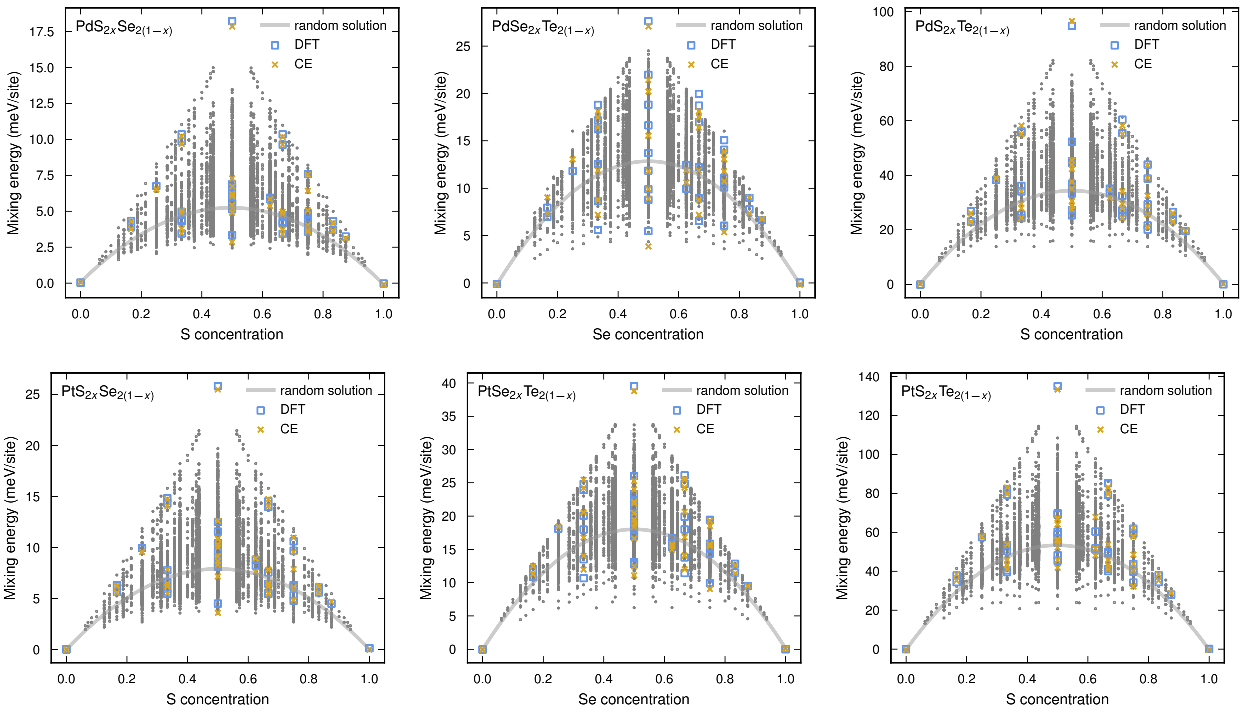


**Figure S10: Mixing energies for Pd/Pt-based X-site mixing (spacegroup 164).** Small gray circles mark mixing energies of enumerated structures obtained using the CE.

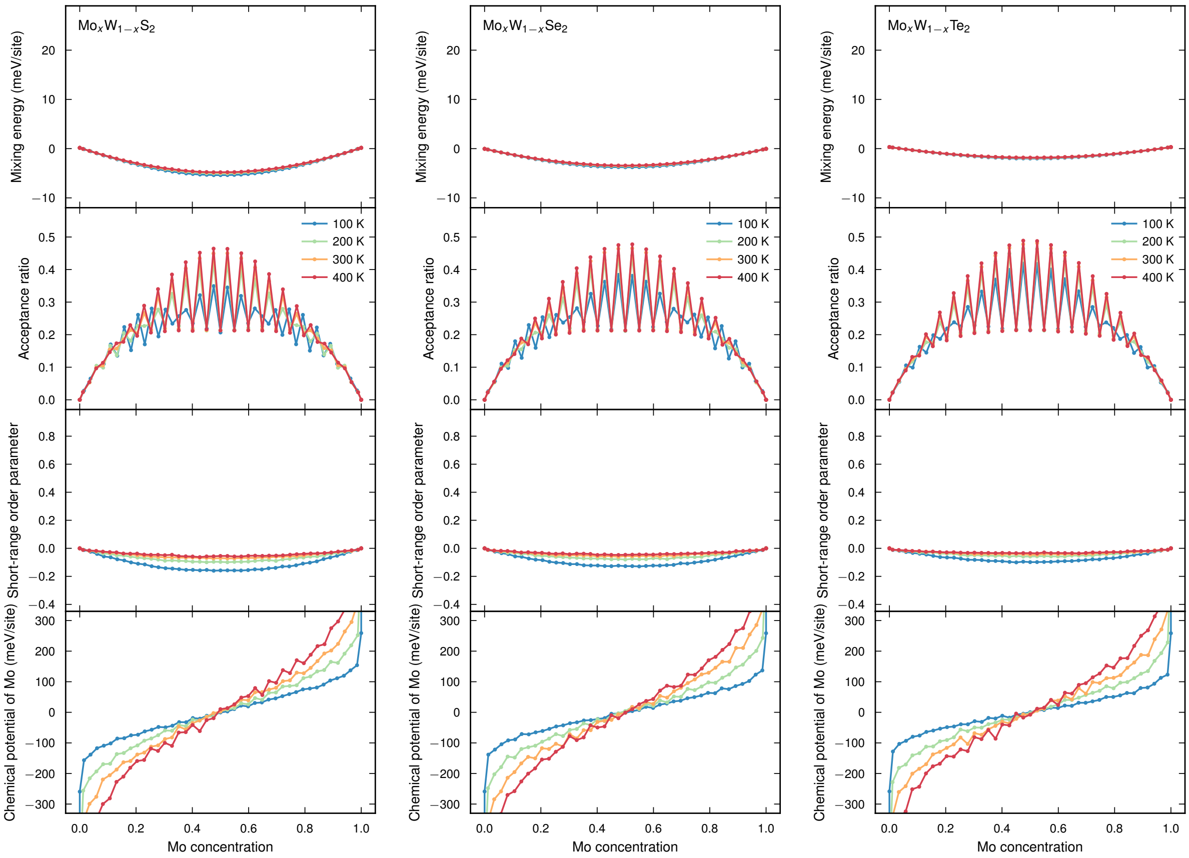


**Figure S11: Results from MC sampling for Mo/W-based M-site mixing (spacegroup 187).** XXX.

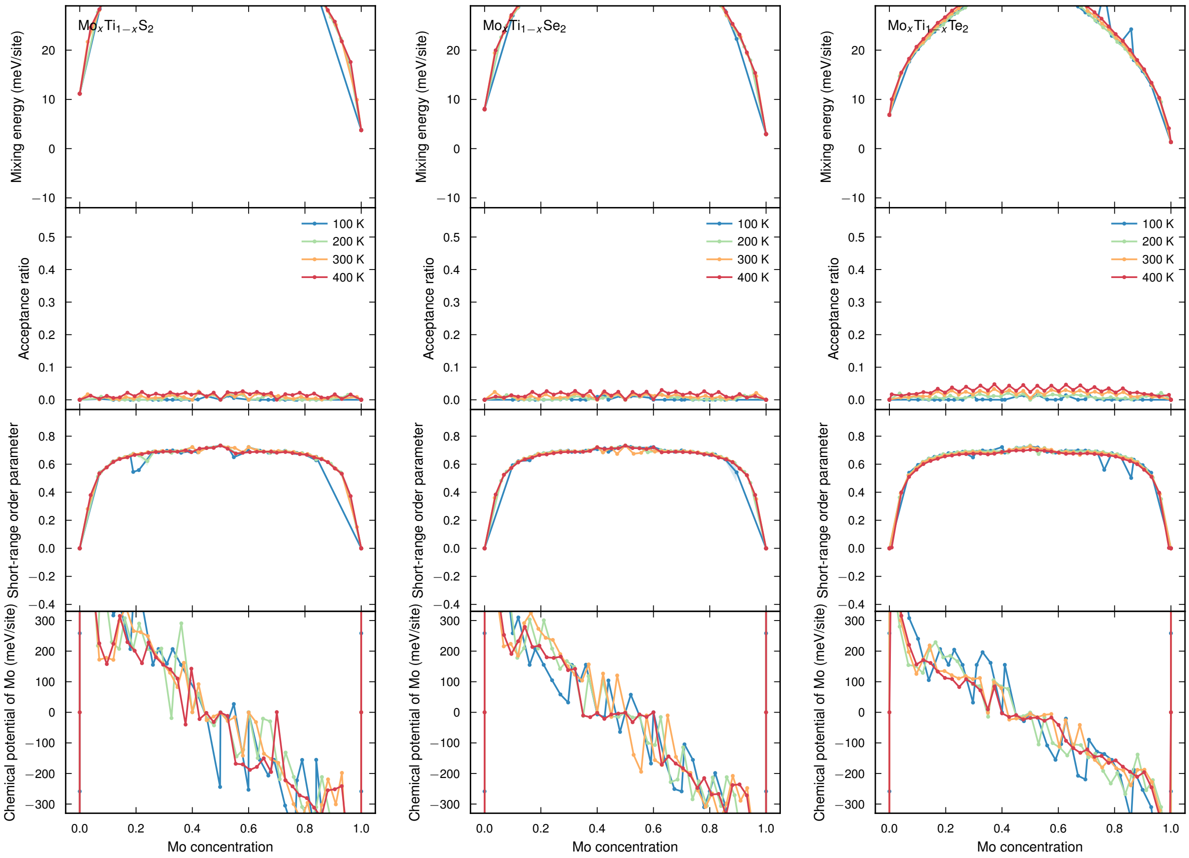


**Figure S12: Results from MC sampling for Mo/Ti-based M-site mixing (spacegroup 187).** XXX.

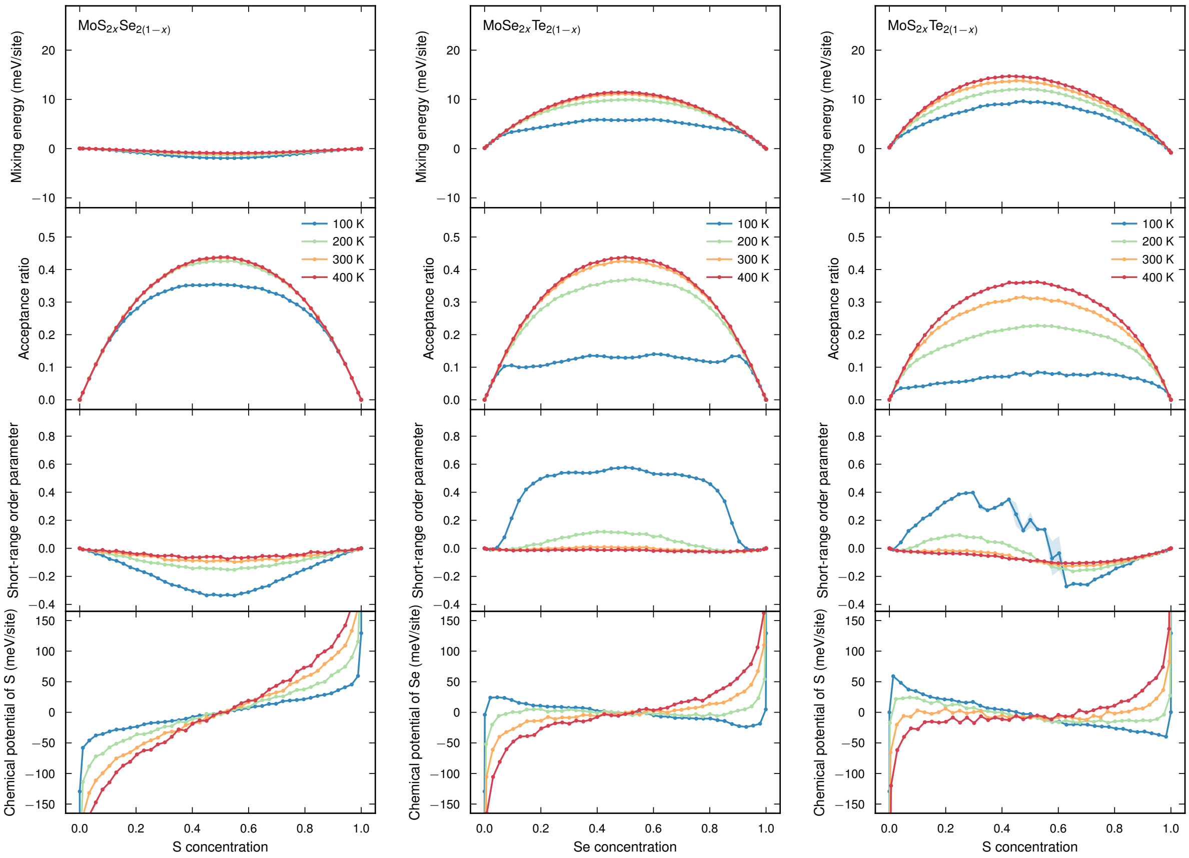


**Figure S13: Results from MC sampling for Mo-based X-site mixing (spacegroup 187).** XXX.

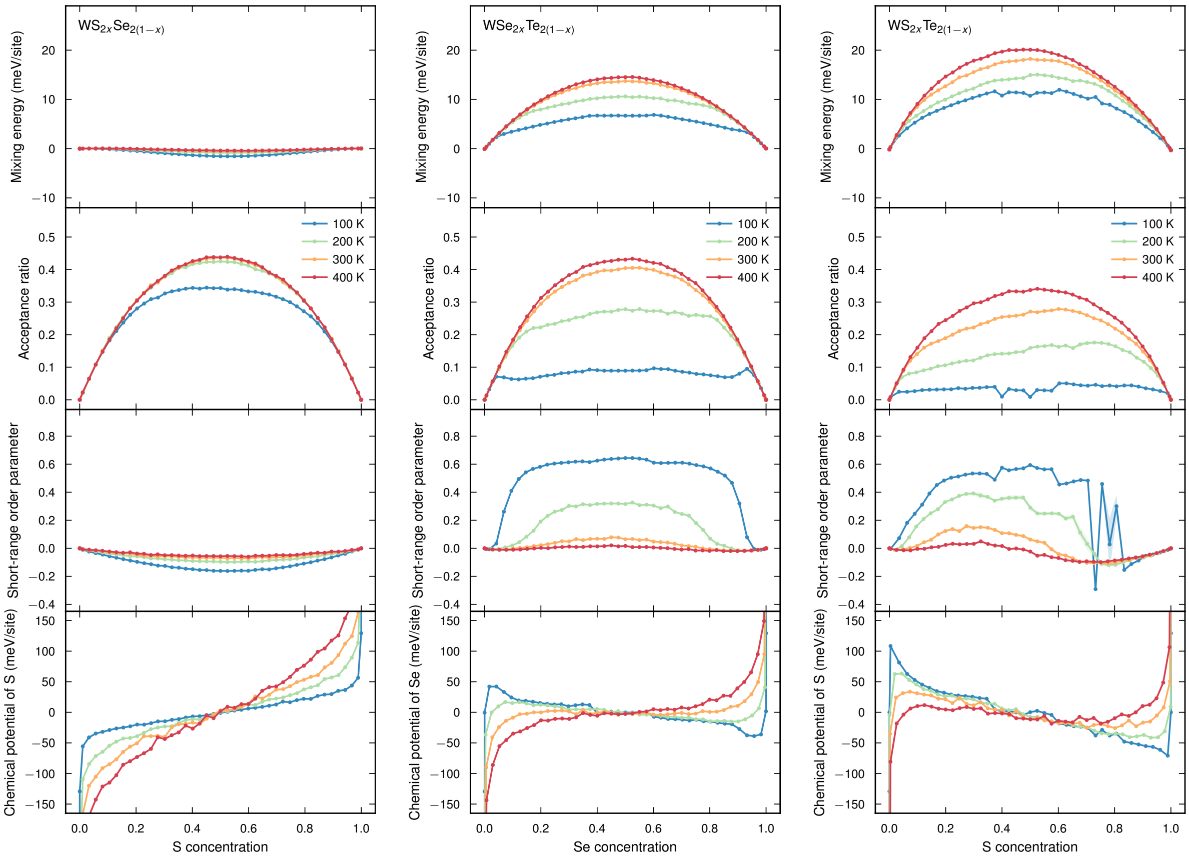


**Figure S14: Results from MC sampling for W-based X-site mixing (spacegroup 187).** XXX.

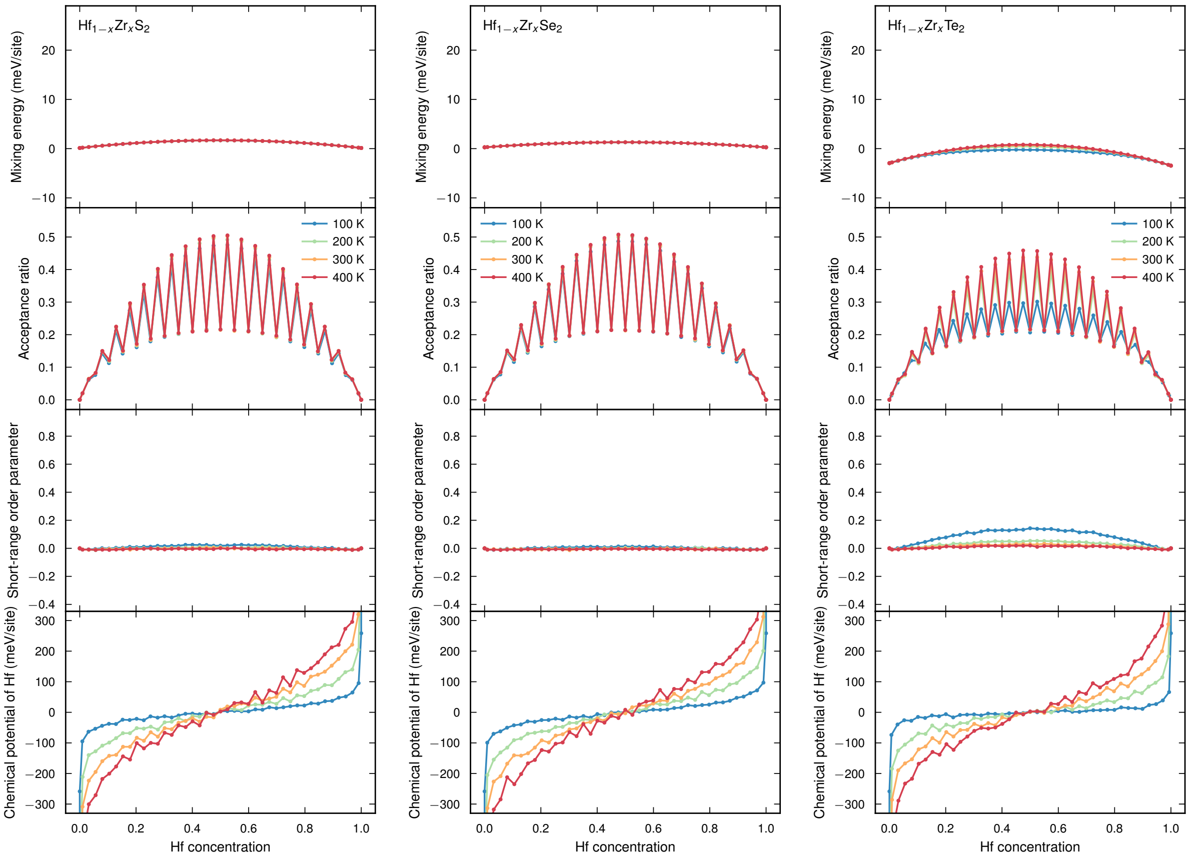


**Figure S15: Results from MC sampling for Hf/Zr-based M-site mixing (spacegroup 164).** XXX.

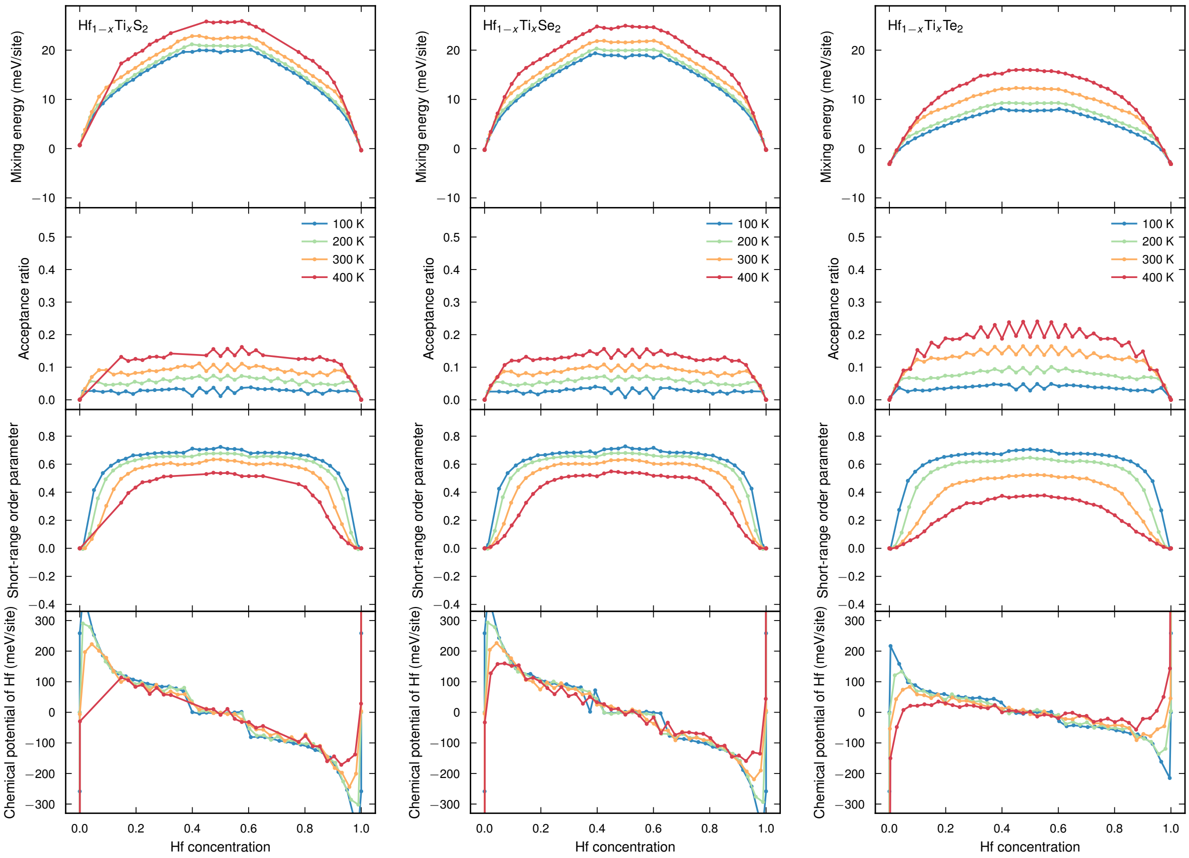


**Figure S16: Results from MC sampling for Hf/Ti-based M-site mixing (spacegroup 164).** XXX.

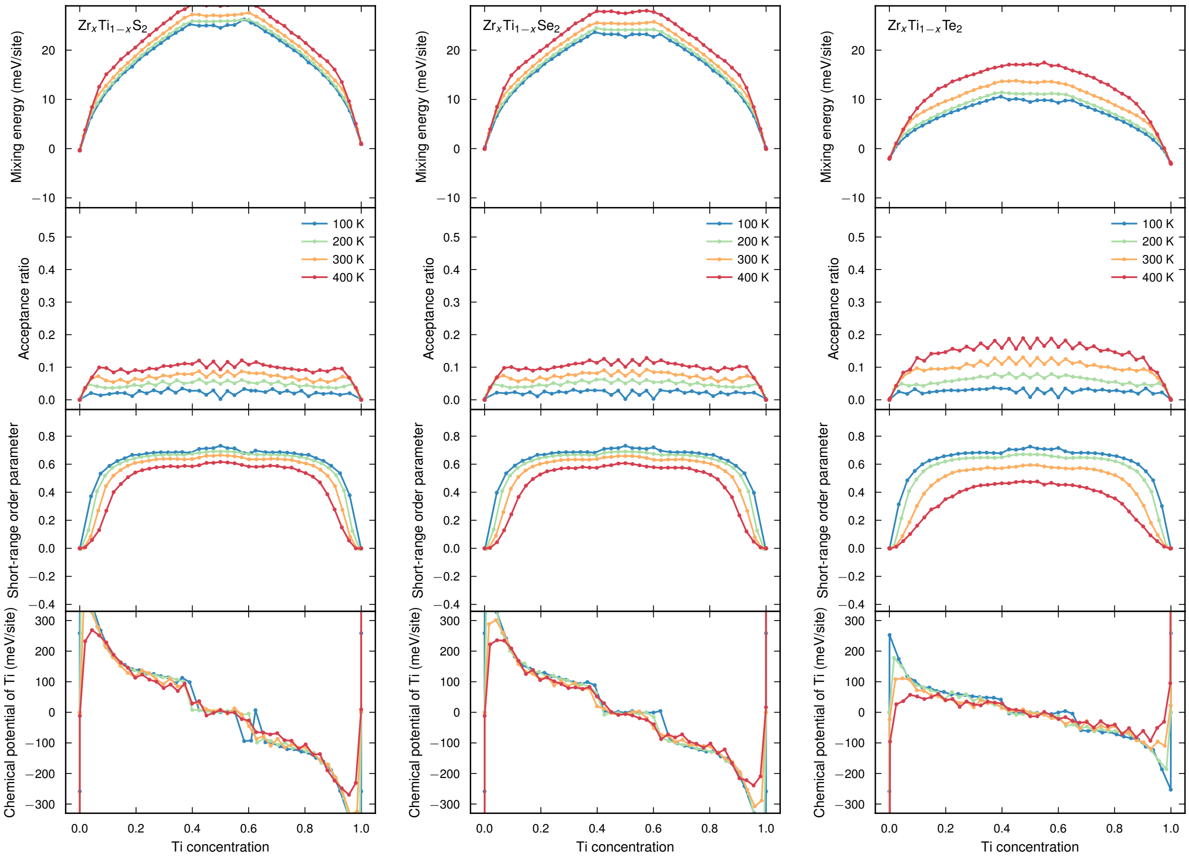


**Figure S17: Results from MC sampling for Ti/Zr-based M-site mixing (spacegroup 164).** XXX.

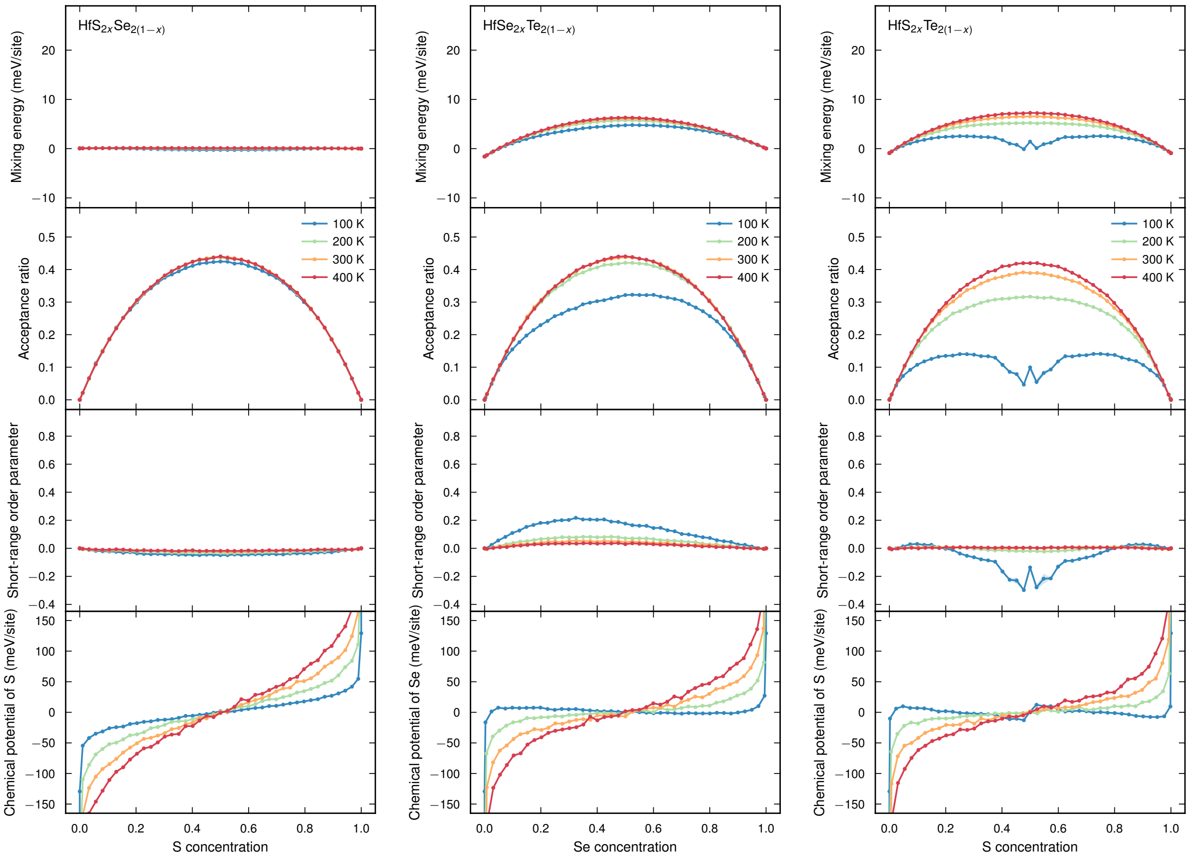


**Figure S18: Results from MC sampling for Hf-based X-site mixing (spacegroup 164).** XXX.

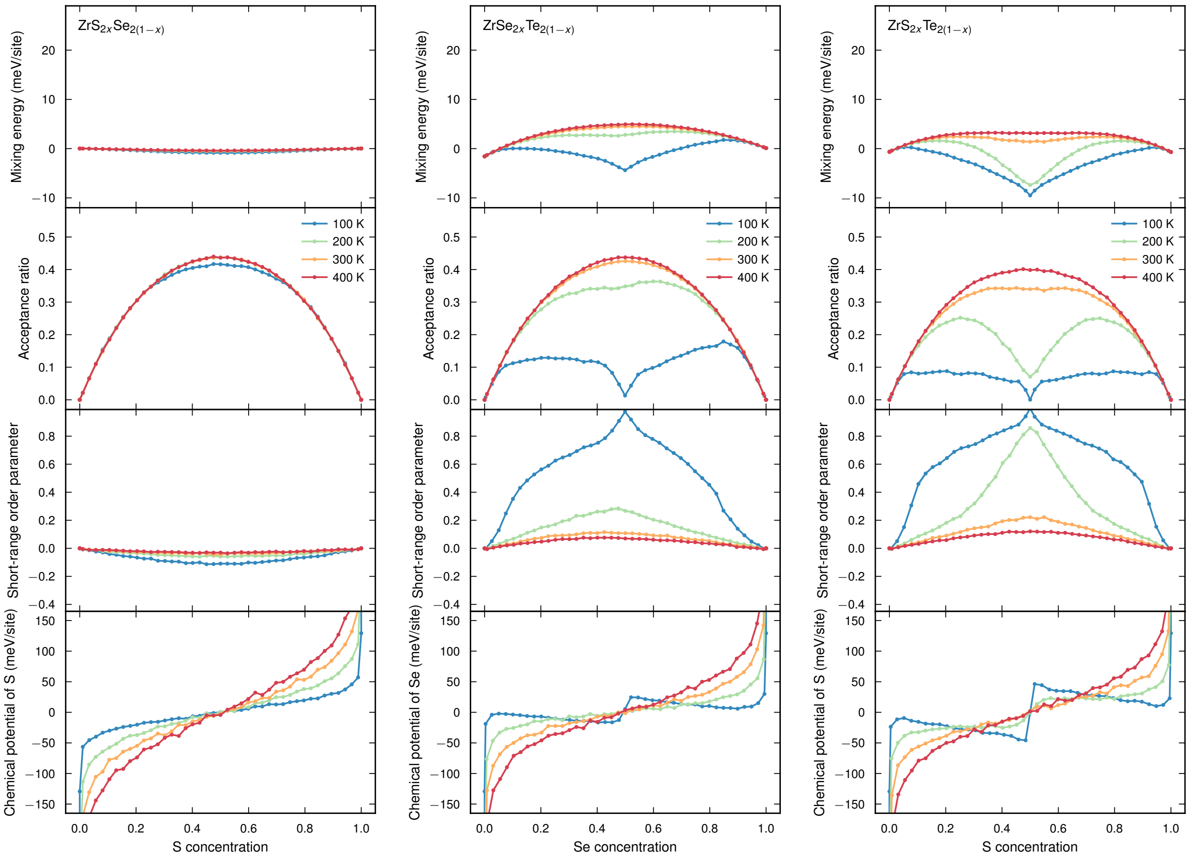


**Figure S19: Results from MC sampling for Zr-based X-site mixing (spacegroup 164).** XXX.

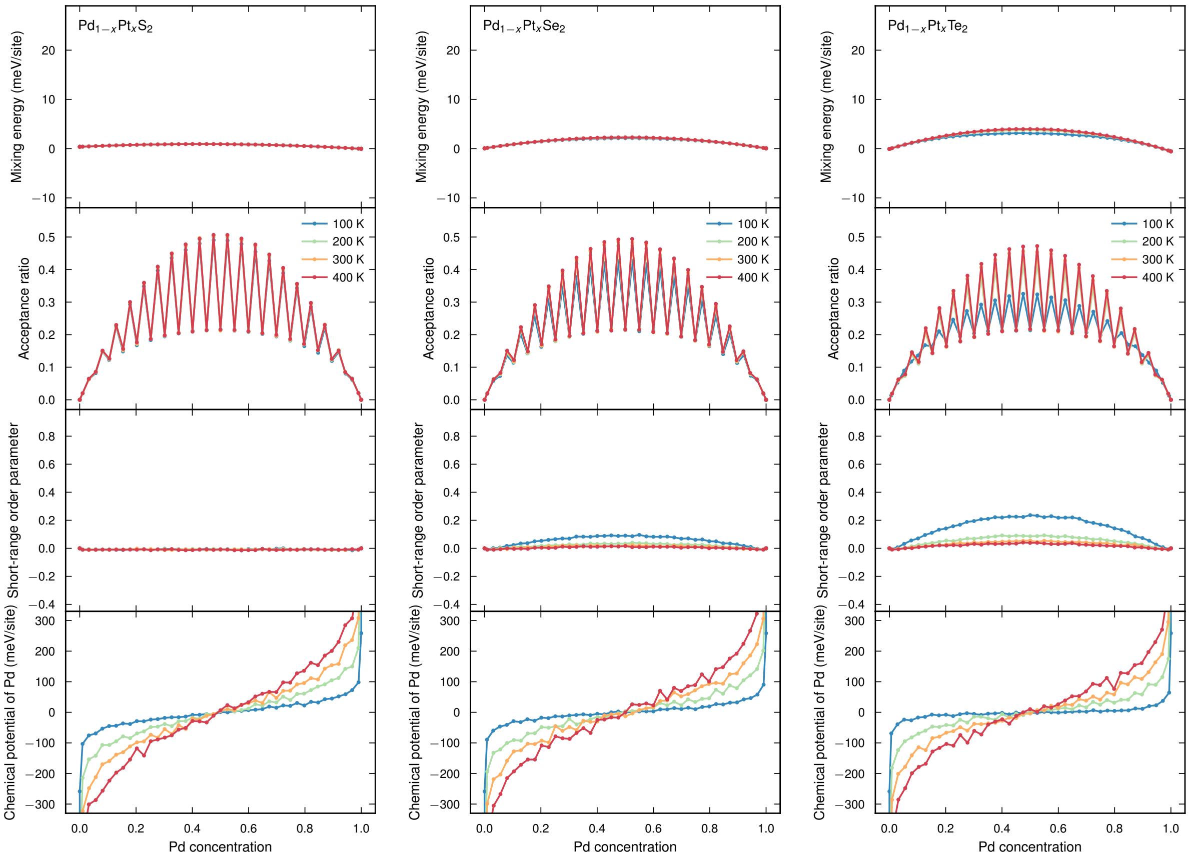


**Figure S20: Results from MC sampling for Pd/Pt-based M-site mixing (spacegroup 164).** XXX.

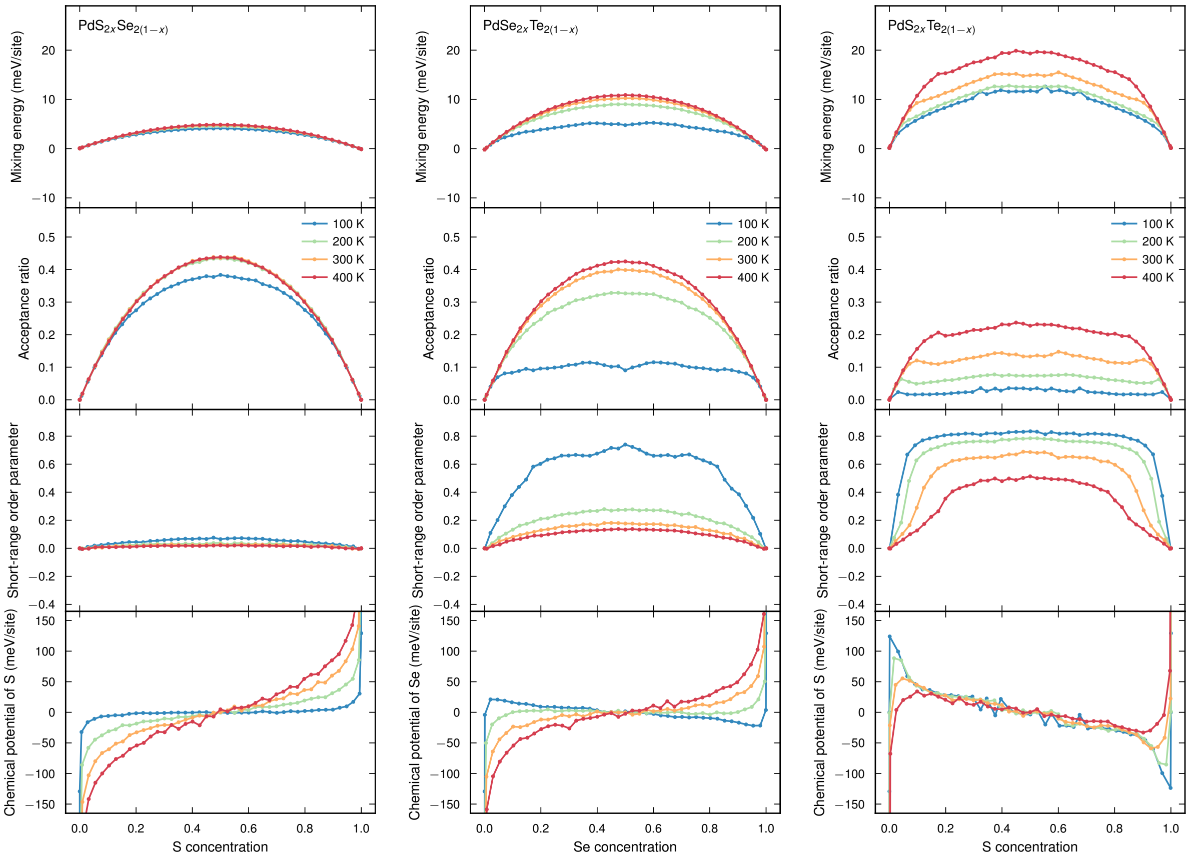


**Figure S21: Results from MC sampling for Pd-based X-site mixing (spacegroup 164).** XXX.

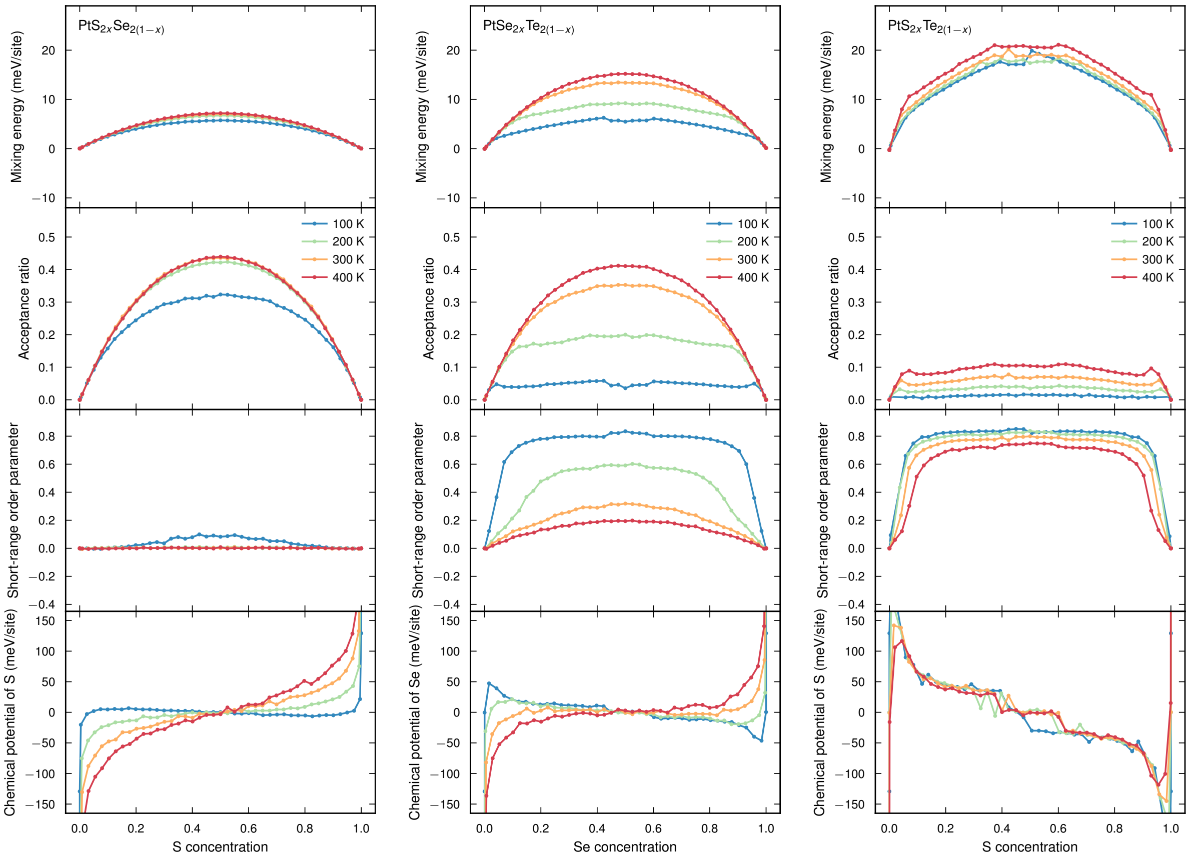


**Figure S22: Results from MC sampling for Pt-based X-site mixing (spacegroup 164).** XXX.

## Supplementary References


[1] Mak, K. F.; Lee, C.; Hone, J.; Shan, J.; Heinz, T. F. Atomically Thin $MoS_2$: A New Direct-Gap Semiconductor. *Physical Review Letters* **2010**, *105*, 136805.

[2] Andersen, K.; Latini, S.; Thygesen, K. S. Dielectric Genome of van der Waals Heterostructures. *Nano Letters* **2015**, *15*, 4616–4621.

[3] Naik, M. H.; Jain, M. Ultraflatbands and Shear Solitons in Moiré Patterns of Twisted Bilayer Transition Metal Dichalcogenides. *Physical Review Letters* **2018**, *121*, 266401.

[4] Brem, S.; Linderälv, C.; Erhart, P.; Malic, E. Tunable Phases of Moiré Excitons in van der Waals Heterostructures. *Nano Letters* **2020**, *20*, 8534–8540.

[5] Hinnemann, B.; Moses, P. G.; Bonde, J.; Jørgensen, K. P.; Nielsen, J. H.; Horch, S.; Chorkendorff, I.; Nørskov, J. K. Biomimetic Hydrogen Evolution: $MoS_2$ Nanoparticles as Catalyst for Hydrogen Evolution. *Journal of the American Chemical Society* **2005**, *127*, 5308–5309.

[6] Yoon, Y.; Ganapathi, K.; Salahuddin, S. How Good Can Monolayer $MoS_2$ Transistors Be? *Nano Letters* **2011**, *11*, 3768–3773.

[7] Radisavljevic, B.; Radenovic, A.; Brivio, J.; Giacometti, V.; Kis, A. Single-layer $MoS_2$ transistors. *Nature Nanotechnology* **2011**, *6*, 147–150.

[8] Yao, J.; Yang, G. 2D Layered Material Alloys: Synthesis and Application in Electronic and Optoelectronic Devices. *Advanced Science* **2022**, *9*, 2103036.

[9] Mleczko, M. J.; Zhang, C.; Lee, H. R.; Kuo, H.-H.; Magyari-Köpe, B.; Moore, R. G.; Shen, Z.-X.; Fisher, I. R.; Nishi, Y.; Pop, E. $HfSe_2$ and $ZrSe_2$: Two-dimensional semiconductors with native high-$\kappa$ oxides. *Science Advances* **2017**, *3*, e1700481.

[10] Wang, J.; Li, Z.; Chen, H.; Deng, G.; Niu, X. Recent Advances in 2D Lateral Heterostructures. *Nano-Micro Letters* **2019**, *11*, 48.

[11] Tang, Q.; Jiang, D.-e. Stabilization and Band-Gap Tuning of the 1T-$MoS_2$ Monolayer by Covalent Functionalization. *Chemistry of Materials* **2015**, *27*, 3743–3748.

[12] Raja, A. et al. Coulomb engineering of the bandgap and excitons in two-dimensional materials. *Nature Communications* **2017**, *8*, 15251.

[13] Padilha, J. E.; Peelaers, H.; Janotti, A.; Van de Walle, C. G. Nature and evolution of the band-edge states in $MoS_2$: From monolayer to bulk. *Physical Review B* **2014**, *90*, 205420.

[14] Riis-Jensen, A. C.; Manti, S.; Thygesen, K. S. Engineering Atomically Sharp Potential Steps and Band Alignment at Solid Interfaces using 2D Janus Layers. *The Journal of Physical Chemistry C* **2020**, *124*, 9572–9580.

[15] Zhang, C.; Li, M.-Y.; Tersoff, J.; Han, Y.; Su, Y.; Li, L.-J.; Muller, D. A.; Shih, C.-K. Strain distributions and their influence on electronic structures of $WSe_2$–$MoS_2$ laterally strained heterojunctions. *Nature Nanotechnology* **2018**, *13*, 152–158.

[16] Conley, H. J.; Wang, B.; Ziegler, J. I.; Haglund, R. F.; Pantelides, S. T.; Bolotin, K. I. Bandgap Engineering of Strained Monolayer and Bilayer $MoS_2$. *Nano Letters* **2013**, *13*, 3626–3630.

[17] Chen, Y.; Xi, J.; Dumcenco, D. O.; Liu, Z.; Suenaga, K.; Wang, D.; Shuai, Z.; Huang, Y.-S.; Xie, L. Tunable Band Gap Photoluminescence from Atomically Thin Transition-Metal Dichalcogenide Alloys. *ACS Nano* **2013**, *7*, 4610–4616.

[18] Komsa, H.-P.; Krasheninnikov, A. V. Two-Dimensional Transition Metal Dichalcogenide Alloys: Stability and Electronic Properties. *The Journal of Physical Chemistry Letters* **2012**, *3*, 3652–3656.

[19] Xie, L. M. Two-dimensional transition metal dichalcogenide alloys: Preparation, characterization and applications. *Nanoscale* **2015**, *7*, 18392–18401.

[20] Kang, J.; Tongay, S.; Li, J.; Wu, J. Monolayer semiconducting transition metal dichalcogenide alloys: Stability and band bowing. *Journal of Applied Physics* **2013**, *113*, 143703.

[21] Kutana, A.; Penev, E. S.; Yakobson, B. I. Engineering electronic properties of layered transition-metal dichalcogenide compounds through alloying. *Nanoscale* **2014**, *6*, 5820–5825.

[22] Yang, J.-H.; Yakobson, B. I. Unusual Negative Formation Enthalpies and Atomic Ordering in Isovalent Alloys of Transition Metal Dichalcogenide Monolayers. *Chemistry of Materials* **2018**, *30*, 1547–1555.

[23] Tan, W.; Wei, Z.; Liu, X.; Liu, J.; Fang, X.; Fang, D.; Wang, X.; Wang, D.; Tang, J.; Fan, X. Ordered and Disordered Phases in $Mo_{1-x}W_xS_2$ Monolayer. *Scientific Reports* **2017**, *7*, 15124.

[24] Duan, X.; Wang, C.; Fan, Z.; Hao, G.; Kou, L.; Halim, U.; Li, H.; Wu, X.; Wang, Y.; Jiang, J.; Pan, A.; Huang, Y.; Yu, R.; Duan, X. Synthesis of $WS_{2x}Se_{2-2x}$ Alloy Nanosheets with Composition-Tunable Electronic Properties. *Nano Letters* **2016**, *16*, 264–269.

[25] Dumcenco, D. O.; Kobayashi, H.; Liu, Z.; Huang, Y.-S.; Suenaga, K. Visualization and quantification of transition metal atomic mixing in $Mo_{1-x}W_xS_2$ single layers. *Nature Communications* **2013**, *4*, 1351.

[26] Xia, X.; Loh, S. M.; Viner, J.; Teutsch, N. C.; Graham, A. J.; Kandyba, V.; Barinov, A.; Sanchez, A. M.; Smith, D. C.; Hine, N. D. M.; Wilson, N. R. Atomic and electronic structure of two-dimensional $Mo_{1-x}W_xS_2$ alloys. *Journal of Physics: Materials* **2021**, *4*, 025004.

[27] Zhang, M.; Zhu, Y.; Wang, X.; Feng, Q.; Qiao, S.; Wen, W.; Chen, Y.; Cui, M.; Zhang, J.; Cai, C.; Xie, L. Controlled Synthesis of $ZrS_2$ Monolayer and Few Layers on Hexagonal Boron Nitride. *Journal of the American Chemical Society* **2015**, *137*, 7051–7054.

[28] Zhao, Y.; Qiao, J.; Yu, P.; Hu, Z.; Lin, Z.; Lau, S. P.; Liu, Z.; Ji, W.; Chai, Y. Extraordinarily Strong Interlayer Interaction in 2D Layered $PtS_2$. *Advanced Materials* **2016**, *28*, 2399–2407.

[29] Haastrup, S.; Strange, M.; Pandey, M.; Deilmann, T.; Schmidt, P. S.; Hinsche, N. F.; Gjerding, M. N.; Torelli, D.; Larsen, P. M.; Riis-Jensen, A. C.; Gath, J.; Jacobsen, K. W.; Mortensen, J.-J.; Olsen, T.; Thygesen, K. S. The Computational 2D Materials Database: High-throughput modeling and discovery of atomically thin crystals. *2D Materials* **2018**, *5*, 042002.

[30] Gjerding, M. N. et al. Recent progress of the computational 2D materials database (C2DB). *2D Materials* **2021**, *8*, 044002.

[31] Lau, K. W.; Cocchi, C.; Draxl, C. Electronic and optical excitations of two-dimensional $ZrS_2$ and $HfS_2$ and their heterostructure. *Physical Review Materials* **2019**, *3*, 074001.

[32] Oliver, S. M.; Fox, J. J.; Hashemi, A.; Singh, A.; Cavalero, R. L.; Yee, S.; Snyder, D. W.; Jaramillo, R.; Komsa, H.-P.; Vora, P. M. Phonons and excitons in $ZrSe_2$–$ZrS_2$ alloys. *J. Mater. Chem. C* **2020**, *8*, 5732–5743.

[33] Gaiser, C.; Zandt, T.; Krapf, A.; Serverin, R.; Janowitz, C.; Manzke, R. Band-gap engineering with $HfS_xSe_{2-x}$. *Physical Review B* **2004**, *69*, 075205.

[34] Moustafa, M.; Zandt, T.; Janowitz, C.; Manzke, R. Growth and band gap determination of the $ZrS_xSe_{2-x}$ single crystal series. *Physical Review B* **2009**, *80*, 035206.

[35] Zhang, J.; Jia, S.; Kholmanov, I.; Dong, L.; Er, D.; Chen, W.; Guo, H.; Jin, Z.; Shenoy, V. B.; Shi, L.; Lou, J. Janus Monolayer Transition-Metal Dichalcogenides. *ACS Nano* **2017**, *11*, 8192–8198.

[36] Lu, A.-Y. et al. Janus monolayers of transition metal dichalcogenides. *Nature Nanotechnology* **2017**, *12*, 744–749.

[37] Ångqvist, M.; Muñoz, W. A.; Rahm, J. M.; Fransson, E.; Durniak, C.; Rozyczko, P.; Rod, T. H.; Erhart, P. ICET – A Python Library for Constructing and Sampling Alloy Cluster Expansions. *Advanced Theory and Simulations* **2019**, *2*, 1900015.

[38] Pedregosa, F. et al. Scikit-learn: Machine Learning in Python. *Journal of Machine Learning Research* **2011**, *12*, 2825–2830.

[39] Blöchl, P. E. Projector augmented-wave method. *Physical Review B* **1994**, *50*, 17953–17979.

[40] Kresse, G.; Hafner, J. Ab initio molecular dynamics for liquid metals. *Physical Review B* **1993**, *47*, 558–561.

[41] Kresse, G.; Furthmüller, J. Efficiency of ab-initio total energy calculations for metals and semiconductors using a plane-wave basis set. *Computational Materials Science* **1996**, *6*, 15–50.

[42] Dion, M.; Rydberg, H.; Schröder, E.; Langreth, D. C.; Lundqvist, B. I. Van der Waals Density Functional for General Geometries. *Physical Review Letters* **2004**, *92*, 246401.

[43] Klimeš, J.; Bowler, D. R.; Michaelides, A. Van der Waals density functionals applied to solids. *Physical Review B* **2011**, *83*, 195131.

[44] Lindroth, D. O.; Erhart, P. Thermal transport in van der Waals solids from first-principles calculations. *Physical Review B* **2016**, *94*, 115205.

[45] Hart, G. L. W.; Forcade, R. W. Algorithm for generating derivative structures. *Physical Review B* **2008**, *77*, 224115.

[46] Cowley, J. M. X-ray measurement of order in single crystals of $Cu_3Au$. *Journal of Applied Physics* **1950**, *21*, 24–30.

[47] Zunger, A.; Wei, S.-H.; Ferreira, L. G.; Bernard, J. E. Special quasirandom structures. *Physical Review Letters* **1990**, *65*, 353.

[48] van de Walle, A.; Tiwary, P.; de Jong, M.; Olmsted, D. L.; Asta, M.; Dick, A.; Shin, D.; Wang, Y.; Chen, L.-Q.; Liu, Z.-K. Efficient stochastic generation of special quasirandom structures. *Calphad* **2013**, *42*, 13.

[49] Berland, K.; Hyldgaard, P. Exchange functional that tests the robustness of the plasmon description of the van der Waals density functional. *Physical Review B* **2014**, *89*, 035412.

[50] Heyd, J.; Scuseria, G. E.; Ernzerhof, M. Hybrid functionals based on a screened Coulomb potential. *Journal of Chemical Physics* **2003**, *118*, 8207–8215, erratum: *ibid.* **124**, 219906 (2006).

[51] Heyd, J.; Scuseria, G. E.; Ernzerhof, M. Hybrid functionals based on a screened Coulomb potential (vol 118, pg 8207, 2003). *Journal of Chemical Physics* **2006**, *124*, 219906.

[52] Hume-Rothery, W.; Mabbott, W., Gilbert; Channel Evans, K. M.; Carpenter, H. C. H. The freezing points, melting points, and solid solubility limits of the alloys of silver and copper with the elements of the B sub-groups. *Philosophical Transactions of the Royal Society of London. Series A, Containing Papers of a Mathematical or Physical Character* **1934**, *233*, 1–97.

[53] Allred, A. Electronegativity values from thermochemical data. *Journal of Inorganic and Nuclear Chemistry* **1961**, *17*, 215–221.

[54] Pike, N. A.; Van Troeye, B.; Dewandre, A.; Petretto, G.; Gonze, X.; Rignanese, G.-M.; Verstraete, M. J. Origin of the counterintuitive dynamic charge in the transition metal dichalcogenides. *Physical Review B* **2017**, *95*, 201106.

[55] Hibino, Y.; Yamazaki, K.; Hashimoto, Y.; Oyanagi, Y.; Sawamoto, N.; Machida, H.; Ishikawa, M.; Sudo, H.; Wakabayashi, H.; Ogura, A. The Physical and Chemical Properties of $MoS_{2(1-x)}Te_{2x}$ Alloy Synthesized by Co-sputtering and Chalcogenization and Their Dependence on Fabrication Conditions. *MRS Advances* **2020**, *5*, 1635–1642.

[56] Sahoo, P. K.; Memaran, S.; Xin, Y.; Balicas, L.; Gutiérrez, H. R. One-pot growth of two-dimensional lateral heterostructures via sequential edge-epitaxy. *Nature* **2018**, *553*, 63–67.

[57] Susarla, S.; Hachtel, J. A.; Yang, X.; Kutana, A.; Apte, A.; Jin, Z.; Vajtai, R.; Idrobo, J. C.; Lou, J.; Yakobson, B. I.; Tiwary, C. S.; Ajayan, P. M. Thermally Induced 2D Alloy-Heterostructure Transformation in Quaternary Alloys. *Advanced Materials* **2018**, *30*, 1804218.

[58] Yuan, J.; Yu, N.; Wang, J.; Xue, K.-H.; Miao, X. Design lateral heterostructure of monolayer $ZrS_2$ and $HfS_2$ from first principles calculations. *Applied Surface Science* **2018**, *436*, 919–926.

[59] Ouyang, R.; Curtarolo, S.; Ahmetcik, E.; Scheffler, M.; Ghiringhelli, L. M. SISSO: A compressed-sensing method for identifying the best low-dimensional descriptor in an immensity of offered candidates. *Physical Review Materials* **2018**, *2*, 083802.
